# Supplementary material for: ICare-DT: a digital twin for continuous forecasting of intensive care patients
Source: arXiv:2611.09712 source file (2026-11-06)
Supplement: Supplementary file 1 [file s2_map.tex]

NaCl $\to$ creatinine & 0.25 & 0.025 & -0.026 & 0.004 & -0.011 & 0.930$^{*}$ \\
NaCl $\to$ creatinine & 0.5 & 0.147$^{*}$ & -0.014 & 0.009 & -0.008 & 0.926$^{*}$ \\
NaCl $\to$ creatinine & 0.75 & 0.253$^{*}$ & 0.006 & 0.019 & -- & 0.920$^{*}$ \\
NaCl $\to$ creatinine & 1 & 0.345$^{*}$ & 0.030 & 0.032 & 0.078 & 0.907$^{*}$ \\
\midrule
Phenylephrine $\to$ heart rate & 0.25 & 0.077 & -0.013 & -0.009 & 0.019 & 0.802$^{*}$ \\
Phenylephrine $\to$ heart rate & 0.5 & 0.212$^{*}$ & 0.006 & 0.030 & 0.095 & 0.802$^{*}$ \\
Phenylephrine $\to$ heart rate & 0.75 & 0.310$^{*}$ & 0.036 & 0.064 & 0.181$^{*}$ & 0.802$^{*}$ \\
Phenylephrine $\to$ heart rate & 1 & 0.385$^{*}$ & 0.073 & 0.115 & 0.254$^{*}$ & 0.802$^{*}$ \\
\midrule
Norepinephrine $\to$ heart rate & 0.25 & 0.089 & -0.026 & 0.004 & -0.001 & 0.675$^{*}$ \\
Norepinephrine $\to$ heart rate & 0.5 & 0.220$^{*}$ & 0.000 & 0.035 & 0.085 & 0.675$^{*}$ \\
Norepinephrine $\to$ heart rate & 0.75 & -- & 0.038 & 0.070 & 0.183$^{*}$ & 0.675$^{*}$ \\
Norepinephrine $\to$ heart rate & 1 & 0.393$^{*}$ & 0.081 & 0.101 & 0.254$^{*}$ & 0.675$^{*}$ \\
