# Supplementary material for: ICare-DT: a digital twin for continuous forecasting of intensive care patients
Source: arXiv:2611.09712 source file (2026-11-06)
Supplement: Supplementary file 2 [file s2x_a_desc.tex]

\spo{} (12, 6) & 96.526 & 0.330 & +0.042 [+0.024, +0.062] & +0.029 [+0.016, +0.040] & +0.014 [+0.008, +0.019] & 0.016 & 0.028 \\
\spo{} (18, 12) & 96.526 & 0.561 & +0.057 [+0.029, +0.084] & $-$0.031 [$-$0.048, $-$0.013] & $-$0.015 [$-$0.023, $-$0.007] & 0.020 & 0.035 \\
\spo{} (30, 24) & 96.526 & 0.665 & +0.020 [$-$0.028, +0.066] & $-$0.012 [$-$0.040, +0.017] & $-$0.007 [$-$0.018, +0.005] & 0.047 & 0.052 \\
Heart rate (12, 6) & 86.776 & 0.161 & +0.088 [+0.066, +0.110] & $-$0.024 [$-$0.036, $-$0.012] & $-$0.007 [$-$0.011, $-$0.004] & 0.008 & 0.011 \\
Heart rate (18, 12) & 86.776 & 0.300 & +0.118 [+0.094, +0.142] & $-$0.064 [$-$0.079, $-$0.049] & $-$0.025 [$-$0.030, $-$0.019] & 0.006 & 0.006 \\
Heart rate (30, 24) & 86.776 & 0.482 & +0.098 [+0.061, +0.136] & $-$0.033 [$-$0.061, $-$0.006] & $-$0.022 [$-$0.032, $-$0.012] & 0.009 & 0.005 \\
Respiratory rate (12, 6) & 20.259 & 0.378 & +0.062 [+0.040, +0.083] & $-$0.020 [$-$0.034, $-$0.005] & $-$0.013 [$-$0.018, $-$0.008] & 0.014 & 0.018 \\
Respiratory rate (18, 12) & 20.259 & 0.610 & +0.057 [+0.029, +0.085] & $-$0.036 [$-$0.056, $-$0.016] & $-$0.021 [$-$0.029, $-$0.013] & 0.014 & 0.040 \\
Respiratory rate (30, 24) & 20.259 & 0.766 & +0.028 [$-$0.028, +0.083] & $-$0.029 [$-$0.062, +0.005] & $-$0.016 [$-$0.030, $-$0.002] & 0.036 & 0.062 \\
