# Supplementary material for: ICare-DT: a digital twin for continuous forecasting of intensive care patients
Source: arXiv:2611.09712 source file (2026-11-06)
Supplement: Supplementary file 3 [file s2x_a_ma3.tex]

Heart rate & 0.865 & 0.466 & 1.85 \\
Respiratory rate & 0.857 & 0.461 & 1.86 \\
\spo{} & 0.850 & 0.456 & 1.86 \\
SaO\textsubscript{2} & 0.025 & 0.012 & 2.18 \\
Non-invasive mean arterial pressure & 0.600 & 0.287 & 2.09 \\
Invasive mean arterial pressure & 0.279 & 0.180 & 1.55 \\
Temperature & 0.261 & 0.139 & 1.88 \\
Urine output & 0.479 & 0.271 & 1.77 \\
Creatinine & 0.076 & 0.060 & 1.27 \\
Lactate & 0.052 & 0.021 & 2.42 \\
pH & 0.077 & 0.036 & 2.15 \\
Partial thromboplastin time & 0.054 & 0.036 & 1.52 \\
\midrule
\multicolumn{4}{l}{Valid test hours in hours 1 to 30: 411,460} \\
