# Supplementary material for: ICare-DT: a digital twin for continuous forecasting of intensive care patients
Source: arXiv:2611.09712 source file (2026-11-06)
Supplement: Supplementary file 4 [file s2x_a_mech.tex]

\spo{} (12, 6) & 2,485 & 2,520 & 0.986 & 5.8 & 81.6 & 0.0 \\
\spo{} (18, 12) & 1,493 & 1,466 & 1.018 & 6.0 & 77.9 & 0.0 \\
\spo{} (30, 24) & 559 & 566 & 0.988 & 6.3 & 66.7 & 0.0 \\
Heart rate (12, 6) & 3,277 & 3,232 & 1.014 & 2.7 & 83.8 & 0.0 \\
Heart rate (18, 12) & 2,066 & 2,019 & 1.023 & 2.9 & 79.8 & 0.0 \\
Heart rate (30, 24) & 876 & 850 & 1.031 & 3.4 & 78.0 & 0.0 \\
Respiratory rate (12, 6) & 2,341 & 2,321 & 1.009 & 3.6 & 84.8 & 0.0 \\
Respiratory rate (18, 12) & 1,227 & 1,226 & 1.001 & 4.1 & 82.3 & 0.0 \\
Respiratory rate (30, 24) & 401 & 380 & 1.055 & 4.2 & 76.1 & 0.0 \\
