# Supplementary material for: ICare-DT: a digital twin for continuous forecasting of intensive care patients
Source: arXiv:2611.09712 source file (2026-11-06)
Supplement: Supplementary file 5 [file s2x_a_primary.tex]

\spo{} (12, 6) & 2,485 & 2,241 & 819 & +0.025$^{*}$ [+0.006, +0.046] & 0.022 & $-$0.084$^{\dagger}$ [$-$0.114, $-$0.053] & 0.0018 & +0.078 / +0.062 & +0.073 / +0.023 \\
\spo{} (18, 12) & 1,493 & 1,387 & 837 & +0.041$^{*}$ [+0.011, +0.071] & 0.022 & $-$0.013 [$-$0.048, +0.023] & 1.0 & +0.101 / +0.060 & +0.083 / +0.025 \\
\spo{} (30, 24) & 559 & 529 & 372 & +0.029 [$-$0.021, +0.077] & 0.26 & $-$0.011 [$-$0.071, +0.048] & 1.0 & +0.153 / +0.085 & +0.136 / +0.017 \\
Heart rate (12, 6) & 3,277 & 2,856 & 527 & +0.088$^{*}$ [+0.066, +0.110] & 0.0018 & $-$0.008 [$-$0.021, +0.005] & 1.0 & +0.116 / +0.010 & -- \\
Heart rate (18, 12) & 2,066 & 1,855 & 620 & +0.114$^{*}$ [+0.092, +0.136] & 0.0018 & +0.001 [$-$0.013, +0.016] & 1.0 & +0.107 / +0.027 & -- \\
Heart rate (30, 24) & 876 & 822 & 422 & +0.111$^{*}$ [+0.077, +0.146] & 0.0018 & $-$0.042$^{\dagger}$ [$-$0.070, $-$0.014] & 0.034 & +0.121 / +0.042 & -- \\
Respiratory rate (12, 6) & 2,341 & 2,106 & 885 & +0.068$^{*}$ [+0.045, +0.089] & 0.0018 & +0.023$^{*}$ [+0.007, +0.039] & 0.030 & +0.102 / +0.048 & -- \\
Respiratory rate (18, 12) & 1,227 & 1,148 & 748 & +0.062$^{*}$ [+0.036, +0.089] & 0.0018 & +0.034 [+0.007, +0.061] & 0.10 & +0.083 / +0.046 & -- \\
Respiratory rate (30, 24) & 401 & 385 & 307 & +0.075$^{*}$ [+0.023, +0.126] & 0.022 & $-$0.030 [$-$0.089, +0.028] & 1.0 & +0.108 / +0.049 & -- \\
