# Supplementary material for: ICare-DT: a digital twin for continuous forecasting of intensive care patients
Source: arXiv:2611.09712 source file (2026-11-06)
Supplement: Supplementary file 6 [file s2x_a_seed.tex]

\spo{} (12, 6) & 13 & 0.604 & 0.574 & 0.556 & 0.675 & +0.030 & $-$0.071 \\
 & 17 & 0.576 & 0.562 & 0.542 & 0.675 & +0.014 & $-$0.099 \\
 & 23 & 0.594 & 0.564 & 0.551 & 0.675 & +0.031 & $-$0.081 \\
 & 29 & 0.593 & 0.569 & 0.560 & 0.675 & +0.024 & $-$0.083 \\
 & 31 & 0.590 & 0.562 & 0.537 & 0.675 & +0.028 & $-$0.085 \\
 & Five-seed mean & 0.592 & 0.566 & 0.549 & 0.675 & +0.025 & $-$0.084 \\
\midrule
\spo{} (18, 12) & 13 & 0.643 & 0.598 & 0.575 & 0.636 & +0.045 & +0.008 \\
 & 17 & 0.610 & 0.569 & 0.561 & 0.636 & +0.041 & $-$0.026 \\
 & 23 & 0.626 & 0.572 & 0.552 & 0.636 & +0.053 & $-$0.010 \\
 & 29 & 0.628 & 0.594 & 0.574 & 0.636 & +0.034 & $-$0.007 \\
 & 31 & 0.608 & 0.575 & 0.567 & 0.636 & +0.033 & $-$0.027 \\
 & Five-seed mean & 0.623 & 0.582 & 0.566 & 0.636 & +0.041 & $-$0.013 \\
\midrule
\spo{} (30, 24) & 13 & 0.638 & 0.585 & 0.601 & 0.622 & +0.053 & +0.015 \\
 & 17 & 0.618 & 0.589 & 0.594 & 0.622 & +0.028 & $-$0.005 \\
 & 23 & 0.608 & 0.567 & 0.570 & 0.622 & +0.041 & $-$0.014 \\
 & 29 & 0.605 & 0.599 & 0.614 & 0.622 & +0.006 & $-$0.017 \\
 & 31 & 0.585 & 0.569 & 0.576 & 0.622 & +0.016 & $-$0.037 \\
 & Five-seed mean & 0.611 & 0.582 & 0.591 & 0.622 & +0.029 & $-$0.011 \\
\midrule
Heart rate (12, 6) & 13 & 0.730 & 0.635 & 0.636 & 0.732 & +0.094 & $-$0.002 \\
 & 17 & 0.719 & 0.633 & 0.634 & 0.732 & +0.086 & $-$0.013 \\
 & 23 & 0.726 & 0.640 & 0.637 & 0.732 & +0.086 & $-$0.006 \\
 & 29 & 0.726 & 0.638 & 0.640 & 0.732 & +0.088 & $-$0.006 \\
 & 31 & 0.720 & 0.634 & 0.633 & 0.732 & +0.086 & $-$0.012 \\
 & Five-seed mean & 0.724 & 0.636 & 0.636 & 0.732 & +0.088 & $-$0.008 \\
\midrule
Heart rate (18, 12) & 13 & 0.731 & 0.617 & 0.616 & 0.732 & +0.113 & $-$0.001 \\
 & 17 & 0.730 & 0.615 & 0.615 & 0.732 & +0.115 & $-$0.001 \\
 & 23 & 0.735 & 0.620 & 0.613 & 0.732 & +0.115 & +0.003 \\
 & 29 & 0.736 & 0.626 & 0.619 & 0.732 & +0.110 & +0.004 \\
 & 31 & 0.732 & 0.616 & 0.611 & 0.732 & +0.116 & 0.000 \\
 & Five-seed mean & 0.733 & 0.619 & 0.615 & 0.732 & +0.114 & +0.001 \\
\midrule
Heart rate (30, 24) & 13 & 0.651 & 0.544 & 0.561 & 0.696 & +0.108 & $-$0.044 \\
 & 17 & 0.656 & 0.546 & 0.558 & 0.696 & +0.110 & $-$0.040 \\
 & 23 & 0.656 & 0.542 & 0.554 & 0.696 & +0.113 & $-$0.040 \\
 & 29 & 0.652 & 0.543 & 0.556 & 0.696 & +0.109 & $-$0.044 \\
 & 31 & 0.655 & 0.539 & 0.551 & 0.696 & +0.116 & $-$0.041 \\
 & Five-seed mean & 0.654 & 0.543 & 0.556 & 0.696 & +0.111 & $-$0.042 \\
\midrule
Respiratory rate (12, 6) & 13 & 0.637 & 0.561 & 0.571 & 0.603 & +0.076 & +0.034 \\
 & 17 & 0.627 & 0.558 & 0.565 & 0.603 & +0.069 & +0.024 \\
 & 23 & 0.624 & 0.561 & 0.560 & 0.603 & +0.062 & +0.021 \\
 & 29 & 0.624 & 0.557 & 0.564 & 0.603 & +0.067 & +0.021 \\
 & 31 & 0.619 & 0.556 & 0.561 & 0.603 & +0.063 & +0.016 \\
 & Five-seed mean & 0.626 & 0.559 & 0.564 & 0.603 & +0.068 & +0.023 \\
\midrule
Respiratory rate (18, 12) & 13 & 0.647 & 0.580 & 0.588 & 0.588 & +0.067 & +0.059 \\
 & 17 & 0.611 & 0.552 & 0.554 & 0.588 & +0.059 & +0.023 \\
 & 23 & 0.614 & 0.555 & 0.554 & 0.588 & +0.059 & +0.027 \\
 & 29 & 0.628 & 0.557 & 0.567 & 0.588 & +0.071 & +0.041 \\
 & 31 & 0.607 & 0.550 & 0.560 & 0.588 & +0.057 & +0.019 \\
 & Five-seed mean & 0.622 & 0.559 & 0.565 & 0.588 & +0.062 & +0.034 \\
\midrule
Respiratory rate (30, 24) & 13 & 0.623 & 0.547 & 0.595 & 0.624 & +0.077 & $-$0.001 \\
 & 17 & 0.588 & 0.517 & 0.557 & 0.624 & +0.072 & $-$0.036 \\
 & 23 & 0.590 & 0.508 & 0.554 & 0.624 & +0.081 & $-$0.035 \\
 & 29 & 0.606 & 0.516 & 0.569 & 0.624 & +0.091 & $-$0.018 \\
 & 31 & 0.562 & 0.507 & 0.552 & 0.624 & +0.054 & $-$0.063 \\
 & Five-seed mean & 0.594 & 0.519 & 0.566 & 0.624 & +0.075 & $-$0.030 \\
