# Supplementary material for: ICare-DT: a digital twin for continuous forecasting of intensive care patients
Source: arXiv:2611.09712 source file (2026-11-06)
Supplement: Supplementary file 7 [file s2x_a_sens.tex]

\multicolumn{8}{l}{\textit{Per-cell rosters (entry at hour $L$ instead of hour 30)}} \\
\spo{} (12, 6) & 2,550 & 2,298 & 845 & +0.024$^{*}$ [+0.004, +0.043] & 0.038 & $-$0.083$^{\dagger}$ [$-$0.113, $-$0.054] & 0.0018 \\
\spo{} (18, 12) & 1,507 & 1,401 & 851 & +0.042$^{*}$ [+0.013, +0.072] & 0.019 & $-$0.012 [$-$0.048, +0.024] & 1.0 \\
\spo{} (30, 24) & 559 & 529 & 372 & +0.029 [$-$0.021, +0.077] & 0.26 & $-$0.011 [$-$0.071, +0.048] & 1.0 \\
Heart rate (12, 6) & 3,408 & 2,962 & 552 & +0.090$^{*}$ [+0.069, +0.111] & 0.0018 & $-$0.006 [$-$0.019, +0.006] & 1.0 \\
Heart rate (18, 12) & 2,082 & 1,869 & 636 & +0.114$^{*}$ [+0.092, +0.135] & 0.0018 & +0.002 [$-$0.012, +0.016] & 1.0 \\
Heart rate (30, 24) & 876 & 822 & 422 & +0.111$^{*}$ [+0.077, +0.146] & 0.0018 & $-$0.042$^{\dagger}$ [$-$0.070, $-$0.014] & 0.034 \\
Respiratory rate (12, 6) & 2,430 & 2,180 & 916 & +0.066$^{*}$ [+0.044, +0.087] & 0.0018 & +0.024$^{*}$ [+0.008, +0.040] & 0.021 \\
Respiratory rate (18, 12) & 1,237 & 1,157 & 758 & +0.061$^{*}$ [+0.035, +0.087] & 0.0018 & +0.033 [+0.005, +0.059] & 0.12 \\
Respiratory rate (30, 24) & 401 & 385 & 307 & +0.075$^{*}$ [+0.023, +0.126] & 0.019 & $-$0.030 [$-$0.089, +0.028] & 1.0 \\
\multicolumn{8}{l}{\textit{Outcome}: \texttt{A\_MAJORITY} (8 of 9 better); \texttt{A2\_CONTRADICTED} (1 of 9 better, 2 worse after correction)} \\
\midrule
\multicolumn{8}{l}{\textit{Thresholds at the eICU-CRD training means (\spo{} 96.520\%, heart rate 85.532 per minute, respiratory rate 20.082 per minute)}} \\
\spo{} (12, 6) & 2,485 & 2,241 & 819 & +0.025$^{*}$ [+0.006, +0.046] & 0.021 & $-$0.084$^{\dagger}$ [$-$0.114, $-$0.053] & 0.0018 \\
\spo{} (18, 12) & 1,493 & 1,387 & 837 & +0.041$^{*}$ [+0.011, +0.071] & 0.019 & $-$0.013 [$-$0.048, +0.023] & 1.0 \\
\spo{} (30, 24) & 559 & 529 & 372 & +0.029 [$-$0.021, +0.077] & 0.26 & $-$0.011 [$-$0.071, +0.048] & 1.0 \\
Heart rate (12, 6) & 3,075 & 2,679 & 520 & +0.081$^{*}$ [+0.060, +0.102] & 0.0018 & $-$0.006 [$-$0.019, +0.007] & 1.0 \\
Heart rate (18, 12) & 1,922 & 1,731 & 614 & +0.111$^{*}$ [+0.088, +0.132] & 0.0018 & +0.003 [$-$0.012, +0.019] & 1.0 \\
Heart rate (30, 24) & 798 & 752 & 390 & +0.100$^{*}$ [+0.064, +0.136] & 0.0018 & $-$0.040$^{\ddagger}$ [$-$0.070, $-$0.009] & 0.080 \\
Respiratory rate (12, 6) & 2,335 & 2,100 & 881 & +0.068$^{*}$ [+0.045, +0.090] & 0.0018 & +0.024$^{*}$ [+0.007, +0.039] & 0.043 \\
Respiratory rate (18, 12) & 1,226 & 1,147 & 748 & +0.062$^{*}$ [+0.035, +0.088] & 0.0018 & +0.034 [+0.008, +0.062] & 0.080 \\
Respiratory rate (30, 24) & 399 & 383 & 305 & +0.076$^{*}$ [+0.025, +0.127] & 0.014 & $-$0.032 [$-$0.090, +0.026] & 1.0 \\
\multicolumn{8}{l}{\textit{Outcome}: \texttt{A\_MAJORITY} (8 of 9 better); \texttt{A2\_CONTRADICTED} (1 of 9 better, 1 worse after correction, 1 worse before correction only)} \\
\midrule
\multicolumn{8}{l}{\textit{Stay-level bootstrap of the eICU-CRD analysis (2,000 replicates, $P$ without the add-one correction)}} \\
\spo{} (12, 6) & 2,485 & 2,241 & 819 & +0.025$^{*}$ [+0.004, +0.046] & 0.046 & $-$0.084$^{\dagger}$ [$-$0.116, $-$0.053] & 0 \\
\spo{} (18, 12) & 1,493 & 1,387 & 837 & +0.041$^{*}$ [+0.013, +0.073] & 0.0080 & $-$0.013 [$-$0.048, +0.022] & 1.0 \\
\spo{} (30, 24) & 559 & 529 & 372 & +0.029 [$-$0.021, +0.078] & 0.25 & $-$0.011 [$-$0.071, +0.051] & 1.0 \\
Heart rate (12, 6) & 3,277 & 2,856 & 527 & +0.088$^{*}$ [+0.067, +0.109] & 0 & $-$0.008 [$-$0.020, +0.004] & 1.0 \\
Heart rate (18, 12) & 2,066 & 1,855 & 620 & +0.114$^{*}$ [+0.092, +0.135] & 0 & +0.001 [$-$0.014, +0.017] & 1.0 \\
Heart rate (30, 24) & 876 & 822 & 422 & +0.111$^{*}$ [+0.077, +0.147] & 0 & $-$0.042$^{\dagger}$ [$-$0.071, $-$0.014] & 0.0080 \\
Respiratory rate (12, 6) & 2,341 & 2,106 & 885 & +0.068$^{*}$ [+0.045, +0.090] & 0 & +0.023$^{*}$ [+0.007, +0.040] & 0.042 \\
Respiratory rate (18, 12) & 1,227 & 1,148 & 748 & +0.062$^{*}$ [+0.036, +0.089] & 0 & +0.034 [+0.006, +0.060] & 0.13 \\
Respiratory rate (30, 24) & 401 & 385 & 307 & +0.075$^{*}$ [+0.024, +0.125] & 0.012 & $-$0.030 [$-$0.090, +0.030] & 1.0 \\
\multicolumn{8}{l}{\textit{Outcome}: \texttt{A\_MAJORITY} (8 of 9 better); \texttt{A2\_CONTRADICTED} (1 of 9 better, 2 worse after correction)} \\
