# Supplementary material for: ICare-DT: a digital twin for continuous forecasting of intensive care patients
Source: arXiv:2611.09712 source file (2026-11-06)
Supplement: Supplementary file 8 [file s2x_a_shift.tex]

Heart rate & 0.466 & 0.587 & 0.79 & $-$0.155 / $-$0.095 \\
Invasive systolic pressure & 0.163 & 0.103 & 1.58 & $-$0.075 / 0.035 \\
Invasive diastolic pressure & 0.163 & 0.103 & 1.58 & $-$0.175 / $-$0.155 \\
Invasive mean arterial pressure & 0.180 & 0.103 & 1.74 & $-$0.155 / $-$0.075 \\
Non-invasive systolic pressure & 0.287 & 0.503 & 0.57 & $-$0.095 / $-$0.085 \\
Non-invasive diastolic pressure & 0.287 & 0.503 & 0.57 & $-$0.125 / $-$0.065 \\
Non-invasive mean arterial pressure & 0.287 & 0.467 & 0.62 & $-$0.115 / $-$0.065 \\
\spo{} & 0.456 & 0.365 & 1.25 & 0.175 / 0.165 \\
SaO\textsubscript{2} & 0.012 & 0.492 & 0.02 & 0.585 / 0.145 \\
Temperature & 0.139 & 0.217 & 0.64 & $-$0.065 / $-$0.045 \\
Respiratory rate & 0.461 & 0.567 & 0.81 & $-$0.215 / $-$0.225 \\
Expiratory tidal volume & 0.025 & 0.015 & 1.69 & 0.195 / $-$0.055 \\
Plateau pressure & 0.018 & 0.015 & 1.23 & $-$0.215 / $-$0.095 \\
Lactate & 0.021 & 0.006 & 3.57 & $-$0.145 / $-$0.195 \\
Blood glucose & 0.123 & 0.158 & 0.78 & $-$0.225 / $-$0.265 \\
Magnesium & 0.058 & 0.023 & 2.46 & $-$0.205 / 0.035 \\
Sodium & 0.066 & 0.046 & 1.42 & $-$0.085 / 0.045 \\
Creatinine & 0.060 & 0.043 & 1.38 & $-$0.365 / $-$0.345 \\
Calcium & 0.053 & 0.042 & 1.26 & $-$0.075 / $-$0.105 \\
Chloride & 0.064 & 0.044 & 1.46 & $-$0.015 / $-$0.005 \\
Potassium & 0.071 & 0.050 & 1.42 & $-$0.185 / $-$0.195 \\
Partial thromboplastin time & 0.036 & 0.008 & 4.37 & $-$0.365 / $-$0.315 \\
Bilirubin & 0.016 & 0.012 & 1.27 & $-$0.275 / $-$0.225 \\
Alanine aminotransferase & 0.016 & 0.012 & 1.26 & $-$0.205 / $-$0.205 \\
Aspartate aminotransferase & 0.016 & 0.013 & 1.26 & $-$0.205 / $-$0.215 \\
Alkaline phosphatase & 0.016 & 0.012 & 1.26 & $-$0.355 / $-$0.325 \\
Albumin & 0.008 & 0.015 & 0.52 & 0.055 / $-$0.025 \\
Phosphate & 0.053 & 0.015 & 3.43 & $-$0.215 / $-$0.195 \\
Bicarbonate & 0.060 & 0.040 & 1.48 & $-$0.095 / 0.005 \\
Blood urea nitrogen & 0.060 & 0.043 & 1.38 & $-$0.335 / $-$0.345 \\
pH & 0.036 & 0.012 & 2.90 & $-$0.025 / $-$0.065 \\
PaO\textsubscript{2} & 0.033 & 0.013 & 2.63 & $-$0.125 / $-$0.225 \\
PaCO\textsubscript{2} & 0.033 & 0.012 & 2.67 & $-$0.115 / $-$0.175 \\
Hemoglobin & 0.055 & 0.043 & 1.27 & 0.005 / $-$0.115 \\
White blood cells & 0.054 & 0.038 & 1.41 & $-$0.145 / $-$0.235 \\
Platelets & 0.055 & 0.038 & 1.43 & $-$0.195 / $-$0.255 \\
Urine output & 0.271 & 0.146 & 1.85 & $-$0.285 / $-$0.255 \\
Glasgow Coma Scale, total & 0.128 & 0.125 & 1.02 & 0.565 / 0.565 \\
Glasgow Coma Scale, eye & 0.129 & 0.107 & 1.21 & 0.435 / 0.415 \\
Glasgow Coma Scale, motor & 0.128 & 0.107 & 1.20 & 0.335 / 0.345 \\
Glasgow Coma Scale, verbal & 0.129 & 0.106 & 1.21 & 0.635 / 0.625 \\
\midrule
\multicolumn{5}{l}{Seeded training samples: MIMIC-IV 5,000 stays (794,043 valid hours); eICU-CRD 5,000 stays (543,162 valid hours)} \\
