# Supplementary material for: ICare-DT: a digital twin for continuous forecasting of intensive care patients
Source: arXiv:2611.09712 source file (2026-11-06)
Supplement: Supplementary file 9 [file s2x_b_arms.tex]

Scored rows & \multicolumn{2}{c}{19,412 rows, 7,278 persons, 3,417 events} & \multicolumn{2}{c}{23,693 rows, 8,295 persons, 2,407 events} & \multicolumn{2}{c}{29,248 rows, 8,922 persons, 715 events} \\
\midrule
$b$, tree seed 13 (primary comparator) & 0.8162 [0.8072, 0.8251] & 0.3655 & 0.8321 [0.8219, 0.8421] & 0.2528 & 0.8499 [0.8326, 0.8660] & 0.0895 \\
$b$, tree seed 17 & 0.8165 [0.8076, 0.8253] & 0.3655 & 0.8325 [0.8224, 0.8426] & 0.2527 & 0.8498 [0.8327, 0.8659] & 0.0896 \\
$b$, tree seed 23 & 0.8159 [0.8071, 0.8247] & 0.3657 & 0.8325 [0.8224, 0.8426] & 0.2528 & 0.8485 [0.8313, 0.8647] & 0.0898 \\
$b$, tree seed 29 & 0.8167 [0.8078, 0.8255] & 0.3653 & 0.8325 [0.8223, 0.8427] & 0.2527 & 0.8491 [0.8319, 0.8650] & 0.0897 \\
$b$, tree seed 31 & 0.8161 [0.8072, 0.8248] & 0.3659 & 0.8322 [0.8221, 0.8423] & 0.2529 & 0.8495 [0.8323, 0.8657] & 0.0896 \\
$b$, mean over the five tree seeds & 0.8163 [0.8073, 0.8251] & 0.3656 & 0.8324 [0.8222, 0.8425] & 0.2528 & 0.8494 [0.8322, 0.8654] & 0.0896 \\
\midrule
$h$, encoder seed 13, tree seed 13 & 0.8179 [0.8091, 0.8268] & 0.3645 & 0.8360 [0.8261, 0.8460] & 0.2505 & 0.8493 [0.8326, 0.8652] & 0.0896 \\
$h$, encoder seed 17, tree seed 13 & 0.8167 [0.8078, 0.8255] & 0.3650 & 0.8345 [0.8244, 0.8444] & 0.2514 & 0.8534 [0.8366, 0.8690] & 0.0891 \\
$h$, encoder seed 23, tree seed 13 & 0.8166 [0.8078, 0.8254] & 0.3651 & 0.8362 [0.8262, 0.8460] & 0.2508 & 0.8507 [0.8339, 0.8665] & 0.0897 \\
$h$, encoder seed 29, tree seed 13 & 0.8172 [0.8085, 0.8261] & 0.3648 & 0.8348 [0.8248, 0.8447] & 0.2513 & 0.8524 [0.8360, 0.8681] & 0.0897 \\
$h$, encoder seed 31, tree seed 13 & 0.8178 [0.8090, 0.8265] & 0.3643 & 0.8366 [0.8268, 0.8465] & 0.2510 & 0.8481 [0.8312, 0.8640] & 0.0897 \\
$h$, five-seed mean (primary) & 0.8172 [0.8085, 0.8261] & 0.3647 & 0.8356 [0.8258, 0.8454] & 0.2510 & 0.8508 [0.8343, 0.8663] & 0.0896 \\
\midrule
$h$, encoder and tree seed 17 & 0.8169 [0.8080, 0.8257] & 0.3650 & 0.8341 [0.8241, 0.8440] & 0.2517 & 0.8526 [0.8358, 0.8683] & 0.0891 \\
$h$, encoder and tree seed 23 & 0.8163 [0.8075, 0.8252] & 0.3651 & 0.8366 [0.8266, 0.8465] & 0.2504 & 0.8513 [0.8345, 0.8670] & 0.0897 \\
$h$, encoder and tree seed 29 & 0.8174 [0.8086, 0.8263] & 0.3646 & 0.8347 [0.8247, 0.8447] & 0.2509 & 0.8523 [0.8357, 0.8679] & 0.0896 \\
$h$, encoder and tree seed 31 & 0.8181 [0.8093, 0.8269] & 0.3641 & 0.8372 [0.8273, 0.8471] & 0.2506 & 0.8497 [0.8329, 0.8656] & 0.0896 \\
$h$, paired tree seeds, mean & 0.8173 [0.8086, 0.8262] & 0.3647 & 0.8357 [0.8258, 0.8456] & 0.2508 & 0.8510 [0.8346, 0.8665] & 0.0895 \\
\midrule
$f$, seed 13 & 0.8015 [0.7923, 0.8108] & 0.3768 & 0.7935 [0.7824, 0.8044] & 0.2737 & 0.8291 [0.8114, 0.8465] & 0.0930 \\
$f$, seed 17 & 0.8016 [0.7925, 0.8108] & 0.3779 & 0.7955 [0.7844, 0.8064] & 0.2727 & 0.8345 [0.8171, 0.8517] & 0.0921 \\
$f$, seed 23 & 0.8020 [0.7928, 0.8112] & 0.3768 & 0.7982 [0.7870, 0.8090] & 0.2715 & 0.8327 [0.8157, 0.8494] & 0.0926 \\
$f$, seed 29 & 0.7998 [0.7905, 0.8092] & 0.3775 & 0.7950 [0.7837, 0.8059] & 0.2728 & 0.8277 [0.8103, 0.8448] & 0.0939 \\
$f$, seed 31 & 0.7987 [0.7895, 0.8079] & 0.3779 & 0.7903 [0.7792, 0.8012] & 0.2759 & 0.8264 [0.8089, 0.8436] & 0.0938 \\
$f$, five-seed mean & 0.8007 [0.7916, 0.8099] & 0.3774 & 0.7945 [0.7835, 0.8051] & 0.2733 & 0.8301 [0.8131, 0.8467] & 0.0931 \\
\midrule
$g$, seed 13 & 0.8127 [0.8037, 0.8215] & 0.3685 & 0.8067 [0.7956, 0.8174] & 0.2666 & 0.8365 [0.8191, 0.8534] & 0.0916 \\
$g$, seed 17 & 0.8022 [0.7930, 0.8114] & 0.3757 & 0.7984 [0.7871, 0.8093] & 0.2711 & 0.8222 [0.8041, 0.8399] & 0.0959 \\
$g$, seed 23 & 0.8020 [0.7928, 0.8110] & 0.3764 & 0.8007 [0.7895, 0.8116] & 0.2691 & 0.8319 [0.8141, 0.8493] & 0.0928 \\
$g$, seed 29 & 0.8027 [0.7934, 0.8118] & 0.3755 & 0.7998 [0.7888, 0.8107] & 0.2701 & 0.8229 [0.8045, 0.8409] & 0.0941 \\
$g$, seed 31 & 0.8071 [0.7982, 0.8160] & 0.3732 & 0.8076 [0.7965, 0.8183] & 0.2665 & 0.8371 [0.8195, 0.8540] & 0.0916 \\
$g$, five-seed mean & 0.8053 [0.7963, 0.8141] & 0.3739 & 0.8027 [0.7917, 0.8133] & 0.2687 & 0.8301 [0.8127, 0.8471] & 0.0932 \\
\midrule
$h$, mean of seeds 23 and 29 & 0.8169 [0.8082, 0.8258] & 0.3649 & 0.8355 [0.8255, 0.8453] & 0.2510 & 0.8515 [0.8350, 0.8671] & 0.0897 \\
$f$, mean of seeds 23 and 29 & 0.8009 [0.7917, 0.8102] & 0.3771 & 0.7966 [0.7854, 0.8073] & 0.2721 & 0.8302 [0.8133, 0.8468] & 0.0932 \\
$g$, mean of seeds 23 and 29 & 0.8023 [0.7931, 0.8114] & 0.3760 & 0.8003 [0.7892, 0.8112] & 0.2696 & 0.8274 [0.8095, 0.8448] & 0.0935 \\
