# Supplementary material for: ICare-DT: a digital twin for continuous forecasting of intensive care patients
Source: arXiv:2611.09712 source file (2026-11-06)
Supplement: Supplementary file 10 [file s2x_b_contr.tex]

\multicolumn{6}{l}{\textit{Hypotension (E2)}} \\
\quad $h-b$, primary test & +0.0010 [$-$0.0012, +0.0033] & 0.18 & 0.18 & $-$0.0007 [$-$0.0023, +0.0008] & +0.0042 [+0.0015, +0.0067] \\
\quad $h-b$, paired tree seeds (sensitivity) & +0.0010 [$-$0.0012, +0.0032] & -- & -- & $-$0.0009 [$-$0.0024, +0.0006] & -- \\
\quad $g-b$ & $-$0.0109 [$-$0.0145, $-$0.0072] & -- & -- & +0.0084 [+0.0057, +0.0111] & $-$0.0044 [$-$0.0079, $-$0.0010] \\
\quad $f-b$ & $-$0.0155 [$-$0.0197, $-$0.0114] & -- & -- & +0.0119 [+0.0090, +0.0149] & -- \\
\quad $f-g$ & $-$0.0046 [$-$0.0067, $-$0.0025] & -- & -- & +0.0035 [+0.0018, +0.0052] & -- \\
\quad $h-b$, seeds 23 and 29 & +0.0007 [$-$0.0016, +0.0030] & -- & -- & $-$0.0005 [$-$0.0021, +0.0011] & -- \\
\quad $g-b$, seeds 23 and 29 & $-$0.0139 [$-$0.0178, $-$0.0100] & -- & -- & +0.0105 [+0.0076, +0.0134] & -- \\
\quad $f-b$, seeds 23 and 29 & $-$0.0153 [$-$0.0196, $-$0.0112] & -- & -- & +0.0117 [+0.0087, +0.0147] & -- \\
\midrule
\multicolumn{6}{l}{\textit{Acute kidney injury (E3)}} \\
\quad $h-b$, primary test & +0.0035$^{*}$ [+0.0007, +0.0065] & 0.0088 & 0.018 & $-$0.0018 [$-$0.0032, $-$0.0006] & +0.0075 [+0.0035, +0.0116] \\
\quad $h-b$, paired tree seeds (sensitivity) & +0.0034 [+0.0006, +0.0062] & -- & -- & $-$0.0020 [$-$0.0033, $-$0.0007] & -- \\
\quad $g-b$ & $-$0.0294 [$-$0.0367, $-$0.0226] & -- & -- & +0.0159 [+0.0129, +0.0191] & $-$0.0209 [$-$0.0291, $-$0.0128] \\
\quad $f-b$ & $-$0.0376 [$-$0.0452, $-$0.0304] & -- & -- & +0.0205 [+0.0172, +0.0240] & -- \\
\quad $f-g$ & $-$0.0082 [$-$0.0116, $-$0.0047] & -- & -- & +0.0046 [+0.0031, +0.0062] & -- \\
\quad $h-b$, seeds 23 and 29 & +0.0034 [+0.0003, +0.0064] & -- & -- & $-$0.0018 [$-$0.0032, $-$0.0004] & -- \\
\quad $g-b$, seeds 23 and 29 & $-$0.0318 [$-$0.0393, $-$0.0249] & -- & -- & +0.0168 [+0.0137, +0.0201] & -- \\
\quad $f-b$, seeds 23 and 29 & $-$0.0355 [$-$0.0430, $-$0.0284] & -- & -- & +0.0193 [+0.0160, +0.0229] & -- \\
\midrule
\multicolumn{6}{l}{\textit{Hypoxemia (E4, secondary)}} \\
\quad $h-b$, primary test & +0.0009 [$-$0.0034, +0.0054] & 0.35 & -- & +0.0001 [$-$0.0005, +0.0007] & +0.0013 [$-$0.0032, +0.0059] \\
\quad $h-b$, paired tree seeds (sensitivity) & +0.0017 [$-$0.0026, +0.0059] & -- & -- & $-$0.0001 [$-$0.0007, +0.0004] & -- \\
\quad $g-b$ & $-$0.0197 [$-$0.0275, $-$0.0118] & -- & -- & +0.0037 [+0.0025, +0.0049] & $-$0.0125 [$-$0.0202, $-$0.0054] \\
\quad $f-b$ & $-$0.0198 [$-$0.0283, $-$0.0112] & -- & -- & +0.0036 [+0.0022, +0.0050] & -- \\
\quad $f-g$ & 0.0000 [$-$0.0051, +0.0050] & -- & -- & $-$0.0001 [$-$0.0010, +0.0008] & -- \\
\quad $h-b$, seeds 23 and 29 & +0.0016 [$-$0.0030, +0.0066] & -- & -- & +0.0002 [$-$0.0004, +0.0008] & -- \\
\quad $g-b$, seeds 23 and 29 & $-$0.0225 [$-$0.0309, $-$0.0139] & -- & -- & +0.0040 [+0.0027, +0.0053] & -- \\
\quad $f-b$, seeds 23 and 29 & $-$0.0197 [$-$0.0287, $-$0.0106] & -- & -- & +0.0038 [+0.0024, +0.0052] & -- \\
