# Supplementary material for: ICare-DT: a digital twin for continuous forecasting of intensive care patients
Source: arXiv:2611.09712 source file (2026-11-06)
Supplement: Supplementary file 11 [file s2x_b_fit.tex]

Hypotension (E2) & 90,610 & 33,878 & 14,925 \\
Acute kidney injury (E3) & 109,782 & 38,575 & 11,109 \\
Hypoxemia (E4, secondary) & 136,085 & 41,721 & 3,132 \\
