# Supplementary material for: ICare-DT: a digital twin for continuous forecasting of intensive care patients
Source: arXiv:2611.09712 source file (2026-11-06)
Supplement: Supplementary file 12 [file s2x_b_guard.tex]

Invasive mean arterial pressure (mmHg) & 76.0 & 0 & 76.5 & 0 \\
Non-invasive mean arterial pressure (mmHg) & 78.0 & 1.6$\times10^{-5}$ & 78.0 & 3.1$\times10^{-5}$ \\
\spo{} (\%) & 97.0 & 0 & 97.0 & 0 \\
Creatinine ($\mu$mol/L) & 88.4 & 5.9$\times10^{-5}$ & 88.4 & 8.2$\times10^{-5}$ \\
