# Supplementary material for: ICare-DT: a digital twin for continuous forecasting of intensive care patients
Source: arXiv:2611.09712 source file (2026-11-06)
Supplement: Supplementary file 13 [file s2x_b_land.tex]

\multicolumn{6}{l}{\textit{Hypotension (E2)}} \\
\quad $b$ (tree seed 13) & 0.8162 & 0.8061 & 0.8068 & 0.8179 & 0.3655 [0.3548, 0.3759] \\
\quad $b$, mean over tree seeds & 0.8163 & 0.8059 & 0.8078 & 0.8160 & 0.3656 [0.3549, 0.3759] \\
\quad $h$, five-seed mean & 0.8172 & 0.8061 & 0.8104 & 0.8154 & 0.3647 [0.3540, 0.3753] \\
\quad $h$, paired tree seeds & 0.8173 & 0.8060 & 0.8106 & 0.8158 & 0.3647 [0.3540, 0.3752] \\
\quad $f$, five-seed mean & 0.8007 & 0.7901 & 0.7899 & 0.7977 & 0.3774 [0.3665, 0.3882] \\
\quad $g$, five-seed mean & 0.8053 & 0.7951 & 0.7954 & 0.8055 & 0.3739 [0.3639, 0.3839] \\
\quad $h-b$ & +0.0010 & 0.0000 & +0.0036 & $-$0.0025 & $-$0.0007 [$-$0.0023, +0.0008] \\
\midrule
\multicolumn{6}{l}{\textit{Acute kidney injury (E3)}} \\
\quad $b$ (tree seed 13) & 0.8321 & 0.8402 & 0.8285 & 0.7888 & 0.2528 [0.2437, 0.2620] \\
\quad $b$, mean over tree seeds & 0.8324 & 0.8406 & 0.8286 & 0.7888 & 0.2528 [0.2437, 0.2620] \\
\quad $h$, five-seed mean & 0.8356 & 0.8418 & 0.8315 & 0.7992 & 0.2510 [0.2419, 0.2603] \\
\quad $h$, paired tree seeds & 0.8357 & 0.8422 & 0.8315 & 0.7985 & 0.2508 [0.2417, 0.2601] \\
\quad $f$, five-seed mean & 0.7945 & 0.8024 & 0.7925 & 0.7348 & 0.2733 [0.2638, 0.2833] \\
\quad $g$, five-seed mean & 0.8027 & 0.8107 & 0.8035 & 0.7375 & 0.2687 [0.2592, 0.2784] \\
\quad $h-b$ & +0.0035 & +0.0016 & +0.0030 & +0.0103 & $-$0.0018 [$-$0.0032, $-$0.0006] \\
\midrule
\multicolumn{6}{l}{\textit{Hypoxemia (E4, secondary)}} \\
\quad $b$ (tree seed 13) & 0.8499 & 0.8504 & 0.8640 & 0.8193 & 0.0895 [0.0829, 0.0963] \\
\quad $b$, mean over tree seeds & 0.8494 & 0.8507 & 0.8631 & 0.8175 & 0.0896 [0.0830, 0.0965] \\
\quad $h$, five-seed mean & 0.8508 & 0.8532 & 0.8644 & 0.8149 & 0.0896 [0.0829, 0.0964] \\
\quad $h$, paired tree seeds & 0.8510 & 0.8534 & 0.8648 & 0.8148 & 0.0895 [0.0829, 0.0964] \\
\quad $f$, five-seed mean & 0.8301 & 0.8346 & 0.8455 & 0.7842 & 0.0931 [0.0861, 0.1002] \\
\quad $g$, five-seed mean & 0.8301 & 0.8344 & 0.8467 & 0.7832 & 0.0932 [0.0868, 0.0998] \\
\quad $h-b$ & +0.0009 & +0.0028 & +0.0004 & $-$0.0044 & +0.0001 [$-$0.0005, +0.0007] \\
