# Supplementary material for: ICare-DT: a digital twin for continuous forecasting of intensive care patients
Source: arXiv:2611.09712 source file (2026-11-06)
Supplement: Supplementary file 14 [file s2x_b_rows.tex]

Hypotension (E2) & 12 & 9,586 & 9,560 & 1.003 & 2,113 & 1,949 & 1.084 & 7,278 \\
Hypotension (E2) & 24 & 6,592 & 6,669 & 0.988 & 989 & 952 & 1.039 & 5,283 \\
Hypotension (E2) & 48 & 3,234 & 3,279 & 0.986 & 315 & 311 & 1.013 & 2,777 \\
Acute kidney injury (E3) & 12 & 10,023 & 9,998 & 1.003 & 1,214 & 1,199 & 1.013 & 7,558 \\
Acute kidney injury (E3) & 24 & 8,893 & 8,916 & 0.997 & 892 & 901 & 0.990 & 6,776 \\
Acute kidney injury (E3) & 48 & 4,777 & 4,722 & 1.012 & 301 & 291 & 1.034 & 3,935 \\
Hypoxemia (E4, secondary) & 12 & 12,648 & 12,669 & 0.998 & 342 & 307 & 1.114 & 8,922 \\
Hypoxemia (E4, secondary) & 24 & 10,348 & 10,362 & 0.999 & 248 & 232 & 1.069 & 7,612 \\
Hypoxemia (E4, secondary) & 48 & 6,252 & 6,267 & 0.998 & 125 & 136 & 0.919 & 4,929 \\
\midrule
\multicolumn{9}{l}{Bootstrap population: 9,623 test persons with a test row; rescued zero-measurement stays excluded: 0 (training split), 0 (test split)} \\
