# Supplementary material for: ICare-DT: a digital twin for continuous forecasting of intensive care patients
Source: arXiv:2611.09712 source file (2026-11-06)
Supplement: Supplementary file 15 [file s2x_b_seed.tex]

Hypotension (E2) & 13 & +0.0017 [$-$0.0009, +0.0044] & $-$0.0035 [$-$0.0072, +0.0002] & $-$0.0147 [$-$0.0192, $-$0.0103] \\
 & 17 & +0.0005 [$-$0.0022, +0.0030] & $-$0.0140 [$-$0.0182, $-$0.0099] & $-$0.0146 [$-$0.0190, $-$0.0103] \\
 & 23 & +0.0004 [$-$0.0021, +0.0029] & $-$0.0142 [$-$0.0182, $-$0.0102] & $-$0.0142 [$-$0.0185, $-$0.0101] \\
 & 29 & +0.0010 [$-$0.0014, +0.0036] & $-$0.0135 [$-$0.0176, $-$0.0094] & $-$0.0164 [$-$0.0209, $-$0.0121] \\
 & 31 & +0.0016 [$-$0.0010, +0.0041] & $-$0.0091 [$-$0.0134, $-$0.0049] & $-$0.0175 [$-$0.0219, $-$0.0131] \\
\midrule
Acute kidney injury (E3) & 13 & +0.0039 [+0.0006, +0.0073] & $-$0.0254 [$-$0.0330, $-$0.0182] & $-$0.0386 [$-$0.0463, $-$0.0312] \\
 & 17 & +0.0024 [$-$0.0007, +0.0056] & $-$0.0337 [$-$0.0414, $-$0.0262] & $-$0.0366 [$-$0.0446, $-$0.0290] \\
 & 23 & +0.0041 [+0.0007, +0.0075] & $-$0.0314 [$-$0.0387, $-$0.0244] & $-$0.0339 [$-$0.0415, $-$0.0266] \\
 & 29 & +0.0027 [$-$0.0005, +0.0059] & $-$0.0322 [$-$0.0399, $-$0.0250] & $-$0.0371 [$-$0.0447, $-$0.0299] \\
 & 31 & +0.0045 [+0.0015, +0.0076] & $-$0.0244 [$-$0.0318, $-$0.0174] & $-$0.0418 [$-$0.0497, $-$0.0340] \\
\midrule
Hypoxemia (E4, secondary) & 13 & $-$0.0005 [$-$0.0057, +0.0048] & $-$0.0133 [$-$0.0213, $-$0.0052] & $-$0.0207 [$-$0.0299, $-$0.0115] \\
 & 17 & +0.0035 [$-$0.0015, +0.0087] & $-$0.0277 [$-$0.0376, $-$0.0179] & $-$0.0153 [$-$0.0247, $-$0.0057] \\
 & 23 & +0.0008 [$-$0.0050, +0.0068] & $-$0.0179 [$-$0.0264, $-$0.0092] & $-$0.0172 [$-$0.0266, $-$0.0079] \\
 & 29 & +0.0025 [$-$0.0022, +0.0073] & $-$0.0270 [$-$0.0365, $-$0.0174] & $-$0.0221 [$-$0.0321, $-$0.0121] \\
 & 31 & $-$0.0017 [$-$0.0069, +0.0035] & $-$0.0128 [$-$0.0207, $-$0.0048] & $-$0.0234 [$-$0.0336, $-$0.0133] \\
