# Supplementary material for: ICare-DT: a digital twin for continuous forecasting of intensive care patients
Source: arXiv:2611.09712 source file (2026-11-06)
Supplement: Supplementary file 16 [file s2x_b_train.tex]

Stopped by & cap & cap & cap & patience & patience & cap & patience & patience & patience & patience \\
Epochs run & 15 & 15 & 15 & 14 & 13 & 15 & 7 & 8 & 7 & 14 \\
Best epoch & 15 & 15 & 15 & 12 & 11 & 14 & 5 & 6 & 5 & 12 \\
Batches clipped per epoch & 212 of 212 & 212 of 212 & 212 of 212 & 212 of 212 & 212 of 212 & 212 of 212 & 212 of 212 & 212 of 212 & 212 of 212 & 212 of 212 \\
\midrule
Epoch 1 & 0.2468 & 0.2478 & 0.2493 & 0.2494 & 0.2476 & 0.2418 & 0.2447 & 0.2450 & 0.2410 & 0.2452 \\
Epoch 2 & 0.2427 & 0.2419 & 0.2437 & 0.2443 & 0.2430 & 0.2347 & 0.2367 & 0.2356 & 0.2354 & 0.2361 \\
Epoch 3 & 0.2413 & 0.2395 & 0.2407 & 0.2412 & 0.2399 & 0.2368 & 0.2370 & 0.2338 & 0.2342 & 0.2373 \\
Epoch 4 & 0.2402 & 0.2368 & 0.2378 & 0.2404 & 0.2385 & 0.2322 & 0.2337 & 0.2343 & 0.2321 & 0.2328 \\
Epoch 5 & 0.2383 & 0.2361 & 0.2365 & 0.2372 & 0.2373 & 0.2303 & 0.2318$^{*}$ & 0.2328 & 0.2308$^{*}$ & 0.2319 \\
Epoch 6 & 0.2371 & 0.2348 & 0.2359 & 0.2368 & 0.2375 & 0.2332 & 0.2318 & 0.2305$^{*}$ & 0.2312 & 0.2331 \\
Epoch 7 & 0.2351 & 0.2347 & 0.2354 & 0.2361 & 0.2348 & 0.2299 & 0.2354 & 0.2313 & 0.2329 & 0.2314 \\
Epoch 8 & 0.2347 & 0.2348 & 0.2361 & 0.2347 & 0.2342 & 0.2306 & -- & 0.2336 & -- & 0.2293 \\
Epoch 9 & 0.2352 & 0.2339 & 0.2337 & 0.2338 & 0.2343 & 0.2290 & -- & -- & -- & 0.2313 \\
Epoch 10 & 0.2341 & 0.2345 & 0.2333 & 0.2347 & 0.2332 & 0.2291 & -- & -- & -- & 0.2289 \\
Epoch 11 & 0.2340 & 0.2334 & 0.2324 & 0.2336 & 0.2322$^{*}$ & 0.2281 & -- & -- & -- & 0.2294 \\
Epoch 12 & 0.2329 & 0.2332 & 0.2314 & 0.2325$^{*}$ & 0.2327 & 0.2281 & -- & -- & -- & 0.2281$^{*}$ \\
Epoch 13 & 0.2322 & 0.2340 & 0.2332 & 0.2326 & 0.2326 & 0.2275 & -- & -- & -- & 0.2282 \\
Epoch 14 & 0.2333 & 0.2319 & 0.2312 & 0.2338 & -- & 0.2274$^{*}$ & -- & -- & -- & 0.2293 \\
Epoch 15 & 0.2321$^{*}$ & 0.2314$^{*}$ & 0.2304$^{*}$ & -- & -- & 0.2294 & -- & -- & -- & -- \\
\midrule
\multicolumn{11}{l}{Every run: 54,102 training stays and an inner early-stopping split of 5,936 stays of 4,213 persons} \\
