# Supplementary material for: ICare-DT: a digital twin for continuous forecasting of intensive care patients
Source: arXiv:2611.09712 source file (2026-11-06)
Supplement: Supplementary file 17 [file s2x_deviations_list.tex]

\begin{description}
\item[D1] \textit{From:} item 9: corrected clock for the MIMIC-IV TEST build. \textit{This read:} legacy root and clock (decision 18 supersedes for this read). \textit{Effect:} native to the frozen encoder and to P1; the legacy clock is not discharge-bounded (D15).
\item[D2] \textit{From:} item 9: binarized dose channels. \textit{This read:} continuous; decision 18 waives for frozen weights, C7 extends to family B. \textit{Effect:} recipe as run.
\item[D3] \textit{From:} item 9: MIMIC-IV TRAIN normalization. \textit{This read:} adopted for both families. \textit{Effect:} z = 0 moves to the MIMIC-IV TRAIN mean (HR 85.53 to 86.78, RR 20.08 to 20.26, \spo{} 96.52 to 96.53); eICU-mean sensitivity.
\item[D4] \textit{From:} item 9: five seeds for main arms and baseline finals. \textit{This read:} A: five; B: five for f, g, h; b one fit (C5, C6). \textit{Effect:} tree-seed spread descriptive.
\item[D5] \textit{From:} item 8: composite primaries as competing-risk CIFs, mortality and LOS as disclosed secondaries. \textit{This read:} decision 18 names the P0 variants E2 and E3 as family B's primaries, and C11 supersedes item 8's composite CIF primaries; item 8's mortality and LOS secondaries are kept (scholar, decision item 19) and are scored from the frozen family-A model at hour 48 (3.11), not from a composite-endpoint model. \textit{Effect:} the read tests the paper's claims, not the plan's model; mortality and LOS are reported as descriptive secondaries with no criterion.
\item[D6] \textit{From:} item 3: C01 mortality-24 excluded. \textit{This read:} C01's 24-hour mortality is not scored; the mortality secondaries use the hour-48 landmark only (3.11); E1 excluded. \textit{Effect:} none.
\item[D7] \textit{From:} item 7 and plan F4. \textit{This read:} IC and SH not run (C1). \textit{Effect:} the isolation statement and personalization stay eICU VAL evidence.
\item[D8] \textit{From:} plan WP11 families F1 to F3; master plan wave 3. \textit{This read:} superseded (the WP9 model was never built). \textit{Effect:} none.
\item[D9] \textit{From:} the eICU v2 inference (2,000 stay-level draws, p without add-one, Holm over 12). \textit{This read:} whole-person 10,000 draws, add-one, Holm over 9; the v2 construction as sensitivity (C3). \textit{Effect:} counts comparable, p finite.
\item[D10] \textit{From:} P1 inference (2,000 draws, gate). \textit{This read:} 10,000 draws, one-sided test with Holm over two (C8). \textit{Effect:} a test the eICU numbers never had.
\item[D11] \textit{From:} P1 recipe. \textit{This read:} as run, except: E1 never labeled (the loss pools three endpoints; the E1 logit, index 0, gets no gradient); P1's early-stopping evaluator refuses an endpoint without labelled inner cells, so a declared copy requires them for E2 to E4 only (2.1); fit set = all MIMIC-IV TRAIN less rescued stays (no TRAIN-tune split); five seeds. \textit{Effect:} the pooled loss and early-stopping weights change; the copy equals P1's function when all four endpoints are labelled.
\item[D12] \textit{From:} v2 calibration on eICU VAL. \textit{This read:} none (C2). \textit{Effect:} no calibrated metric.
\item[D13] \textit{From:} v2 built labels in the prediction pass. \textit{This read:} separate label stage after the freeze. \textit{Effect:} seal is by stage, not only by procedure.
\item[D14] \textit{From:} eICU terminal contract (unit discharge offset and status). \textit{This read:} MIMIC-IV contract: ceil of ICU LOS hours; hospital death flag, not an ICU death; exits merged. \textit{Effect:} the family-A and family-B labels code both exits 0, so they are invariant to the cause; of the secondaries, LOS-X\_H uses the clock only and MORT-W and MORT-H read the flag as hospital death (D28).
\item[D15] \textit{From:} legacy clock after the terminal. \textit{This read:} 75.2 \% of MIMIC-IV TRAIN stays have a defining channel measured after the terminal clock (eICU TRAIN-fit 58.5 \%); labels stop at the terminal; a record can reach hour 30 through rows after the terminal. \textit{Effect:} disclosed; the hour-30 entry can include such stays.
\item[D16] \textit{From:} input distribution of the frozen model. \textit{This read:} MIMIC-IV observed-hour ratio to eICU: arterial saturation 0.02 (1.2 \% of hours against 49.2 \%), heart rate 0.79, non-invasive MAP 0.62, most laboratory values 1.4 to 4.4; no remapping (C9). \textit{Effect:} a transfer failure is possible and is reported as such.
\item[D17] \textit{From:} 12 eICU settings. \textit{This read:} 9 (arterial saturation excluded). \textit{Effect:} Holm over 9.
\item[D18] \textit{From:} producer v2's encoding-equality check. \textit{This read:} replaced by explicit pins (3.1). \textit{Effect:} declared exception.
\item[D19] \textit{From:} zero-prior-read TEST authorities. \textit{This read:} the disclosure schema of 7.2. \textit{Effect:} prior reads bound, not denied.
\item[D20] \textit{From:} the v2 bundle committed a stay-level lock. \textit{This read:} nothing stay-level committed (7.8). \textit{Effect:} none.
\item[D21] \textit{From:} E4 channel. \textit{This read:} hourly bedside \spo{} in MIMIC-IV against nurse-charted \spo{} in eICU. \textit{Effect:} different ascertainment.
\item[D22] \textit{From:} eICU TRAIN-tune persons were seen by the pretrained encoder. \textit{This read:} MIMIC-IV persons were not. \textit{Effect:} the tilt in favor of f and h is gone.
\item[D23] \textit{From:} eICU TRAIN-fit 119,330 stays. \textit{This read:} MIMIC-IV TRAIN 66,007. \textit{Effect:} smaller fit set for every arm.
\item[D24] \textit{From:} WP8a used per-cell rosters as primary. \textit{This read:} hour-30 rosters primary, as the paper's headline; per-cell as sensitivity. \textit{Effect:} none.
\item[D25] \textit{From:} the eICU last-value producer computed LOCF for roster stays only and skipped stays without a reading. \textit{This read:} LOCF computed in the predict stage for every stay reaching L, with a missing flag; the roster is applied at scoring. \textit{Effect:} the scored LOCF values are the same computation on the same roster stays.
\item[D26] \textit{From:} P0 ran the physical-unit guard and invalid-value rule on TRAIN only. \textit{This read:} also on TEST, in the label stage. \textit{Effect:} an additional check; a TEST failure stops family B only (C12).
\item[D27] \textit{From:} P0/P1 and the paper's eICU contrast used one tree seed. \textit{This read:} primary unchanged (C6); paired tree-seed sensitivity and the b range added. \textit{Effect:} seed dependence is visible, not tested.
\item[D28] \textit{From:} the eICU death forecast was scored against death in the unit within 48 hours of hour 48 (\texttt{revision\_\allowbreak{}v3\_\allowbreak{}joint\_\allowbreak{}factual\_\allowbreak{}export.\allowbreak{}py:\allowbreak{}228-\allowbreak{}229}). \textit{This read:} MORT-W: hospital death with unit exit within 48 hours; MORT-H: hospital death at any time (3.11). \textit{Effect:} MIMIC-IV records the time of in-hospital death, but the legacy harmonized root used here keeps only a hospital death flag without a time, and this read adds no exporter (4.1); MORT-W contains the eICU label and adds stays that left the unit alive in the window and died later in the hospital; the death forecast targets death in the unit before the head's crossing, so a mean below either observed rate arises in part by construction, as it did against the eICU label; the text states the mean forecast against the observed rate (below, above or within sampling variation), gives that reason only with a shortfall, keeps AUROC as the headline, and 9.3 rewords the paper's eICU sentence to the same standard (3.11).
\item[D29] \textit{From:} the earlier hospital-mortality reads at C = 48 h: corrected clock and LOS $\geq$ 48 h (TRB-M4-20, 7,016 stays of 5,446 persons), or the legacy clock (legacy reads), with models trained on MIMIC-IV. \textit{This read:} legacy clock; terminal clock $>$ 48 and a record reaching hour 48; the frozen eICU model. \textit{Effect:} the same outcome in a population defined by a different clock and entry rule; its size and its overlap with the TRB-M4-20 stays are not known before the read (SC counts it after the marker, 3.11, and the result reports it); no model comparison is made or tested.
\item[D30] \textit{From:} the earlier LOS reads regressed remaining ICU LOS (TRB-M4-21; legacy \texttt{los\_\allowbreak{}h} cells). \textit{This read:} leaving the unit within 6, 12, 24 or 48 hours of hour 48, from the merged-exit forecast (3.11). \textit{Effect:} a threshold of remaining LOS; not comparable with their absolute errors; the exit forecast targets leaving the unit before the head's crossing, a part of every exit, so a mean below the observed rate arises in part by construction (3.11).
\item[D31] \textit{From:} the eICU export read the forecasts at position 48 of one pass over the whole record (\texttt{revision\_\allowbreak{}v3\_\allowbreak{}joint\_\allowbreak{}factual\_\allowbreak{}export.\allowbreak{}py:\allowbreak{}449-\allowbreak{}459}, \texttt{:\allowbreak{}175}). \textit{This read:} one pass over the 48-hour prefix, in the allowlist view of stage AS. \textit{Effect:} the same computation under causal masking, up to floating-point order; test (ii) of 7.3 checks that nothing after hour 48 is read.
\item[D32] \textit{From:} the eICU death interval: five-seed mean with a t interval across seeds, and 2,000 per-seed person draws (\texttt{revision\_\allowbreak{}v3\_\allowbreak{}joint\_\allowbreak{}factual\_\allowbreak{}postprocess.\allowbreak{}py:\allowbreak{}42-\allowbreak{}45}). \textit{This read:} the same t interval, plus 10,000 whole-person draws of the five-seed mean. \textit{Effect:} the paper prints the whole-person interval, which includes sampling of patients; the across-seed interval is in the Supplementary Information.
\end{description}
