# Supplementary material for: ICare-DT: a digital twin for continuous forecasting of intensive care patients
Source: arXiv:2611.09712 source file (2026-11-06)
Supplement: Supplementary file 18 [file s2x_disclosure.tex]

REG-5227 & \texttt{TEST\_\allowbreak{}READ\_\allowbreak{}REGISTRY.\allowbreak{}md:\allowbreak{}14} & 5227 (re-export of the job-2754 aggregate) & 2026-08-09 & previously opened Track B aggregate cells (mortality, LOS) \\
REG-C01 & \texttt{TEST\_\allowbreak{}READ\_\allowbreak{}REGISTRY.\allowbreak{}md:\allowbreak{}24} & 5896-5898 & 2026-08-10 & mortality at 24 h of MIMIC-IV fine-tunes of the same joint lineage (parent seed 29, selection \texttt{744fe1a1}); C01 preparation also read TEST features for eligibility \\
TRB-M4-01 & \texttt{:\allowbreak{}66} & not recorded & 2026-05-23 to 05-27 & mortality and LOS at 6/12/24/48 h; legacy onsets (AKI, hypotension, hypoxemia, lactate, vasopressor start) \\
TRB-M4-02 & \texttt{:\allowbreak{}67} & 2674 & 2026-06-05 & legacy events (SBP $<$ 90, \spo{} $<$ 90, HR $>$ 130); legacy onsets; mortality; LOS \\
TRB-M4-03 & \texttt{:\allowbreak{}68} & 2694 & 2026-06 & as TRB-M4-02 (metrics at least) \\
TRB-M4-04 & \texttt{:\allowbreak{}69} & 2731 & 2026-06-10 & legacy events and onsets; mortality 6 and 24 h; LOS \\
TRB-M4-05 & \texttt{:\allowbreak{}70} & 2711, 2752, 2883, 2754 & 2026-06-07 to 06-14 & mortality and LOS; sensitivity onset cells \\
TRB-M4-06 & \texttt{:\allowbreak{}71} & 3018\_[108-116] & 2026-06-15 & raw future values of the regression targets, including heart rate and respiratory rate, at 1/6/12/24/48 h \\
TRB-M4-07 & \texttt{:\allowbreak{}72} & 3321-3326 & 2026-06 & zero-shot transfer of a frozen eICU twin (A0\_dyn, arm P0) and its online refinement: legacy events, onsets, mortality, LOS \\
TRB-M4-08 & \texttt{:\allowbreak{}73} & 3346-3351 & 2026-06 & legacy events, onsets, mortality, LOS \\
TRB-M4-09 & \texttt{:\allowbreak{}74} & 3468, 3469 & 2026-07-03 & mortality, LOS, strict incident onsets (hypotension, hypoxemia, lactate, AKI, sepsis proxy) at 6/12/24/48 h \\
TRB-M4-10 & \texttt{:\allowbreak{}75} & 3499, 3500, 3574, 3595 & 2026-07 & the same 28-task grid, eICU-trained baselines \\
TRB-M4-11 & \texttt{:\allowbreak{}76} & 3501-3504 & 2026-07 & legacy events, onsets, mortality, LOS \\
TRB-M4-12 & \texttt{:\allowbreak{}77} & 3575, 3601 & 2026-07 & the 28-task grid, target-trained baselines \\
TRB-M4-13 & \texttt{:\allowbreak{}78} & 3534-3539 & 2026-07 & zero-shot transfer of a frozen eICU twin (A0\_dyn\_thr, arm P0) and its online refinement: legacy events, onsets, mortality, LOS \\
TRB-M4-14 & \texttt{:\allowbreak{}79} & 3541, 3542 & 2026-07 & a frozen eICU twin transfer (A0\_dyn, arm P0) and its refinement by stratum \\
TRB-M4-15 & \texttt{:\allowbreak{}80} & 3546 & 2026-07-10 & the frozen eICU twin transfer of TRB-M4-13 by stratum \\
TRB-M4-16 & \texttt{:\allowbreak{}81} & 3586-3591 & 2026-07-10 & zero-shot transfer of a frozen eICU twin (A0\_dyn\_thr, arm P0) with a threshold-calibration rescue: legacy events, onsets, mortality, LOS; closed negative \\
TRB-M4-17 & \texttt{:\allowbreak{}82} & 3621, 3622 & 2026-07-10 & mortality, LOS, lactate and sepsis onset at 24 h \\
TRB-M4-18 & \texttt{:\allowbreak{}83} & 3647-3650, 3809, 3899 & 2026-07-11 on & the same four tasks \\
TRB-M4-19 & \texttt{:\allowbreak{}84} & 4280-4282, 4287-4291, 4300 & 2026-07-21 to 07-23 & the same four tasks \\
TRB-M4-20 & \texttt{:\allowbreak{}85} & 7422-7445 & 2026-08-26 & hospital mortality among stays with LOS $\geq$ C, corrected clock \\
TRB-M4-21 & \texttt{:\allowbreak{}86} & 7451, 7452 & 2026-08-26 & remaining ICU LOS; counted 14,209 finite-LOS stays of 9,804 persons and 2 non-finite \\
TRB-M4-22 & \texttt{:\allowbreak{}87} & 10733 (MIMIC-IV), 10731 (MIMIC-III) & 2026-09-19 & zero-shot transfer of a frozen eICU twin (legacy A0\_dyn): legacy events, onsets, mortality, LOS; null after Holm \\
TRB-M4-23 & \texttt{:\allowbreak{}88} & 10734, 10732 & 2026-09-19 to 09-20 & crossed fine-tune cell, legacy readout \\
TRB-M4-24 & \texttt{:\allowbreak{}89} & not recorded & 2026-05-23 to 05-25 & online personalization D1/D3: legacy events, mortality, onsets \\
TRB-M4-25 & \texttt{:\allowbreak{}90} & not recorded & 2026-05-22 to 05-23 & semi-synthetic MIMIC-IV root generated from TEST covariates \\
TRB-NR-01 & \texttt{:\allowbreak{}91} & 10711, 10712, 10719, 10720, 10725, 10726 & 2026-09-19 & nothing (failed at launch) \\
TRB-NR-02 & \texttt{:\allowbreak{}92} & 10065-10067 & 2026-09-02 & nothing (fit role only) \\
TRB-NR-03 & \texttt{:\allowbreak{}93} & 10535 & 2026-09-12 & nothing on TEST (V\_select only) \\
ID-12997 & \texttt{run\_\allowbreak{}registry.\allowbreak{}csv:\allowbreak{}193} & 12997 & 2026-09-28 & identity columns (\texttt{patient}, \texttt{uniquepid}, split, source) of every label row, TEST included, to select eICU TRAIN \\
ID-13062 & run\_registry row \texttt{V3-\allowbreak{}MIMIC4-\allowbreak{}TRAIN-\allowbreak{}CENSUS-\allowbreak{}32de53f150ae-\allowbreak{}13062} & 13062 & 2026-09-30 & the unchanged normalization verifier read patient, split and source of every label row, and the loader read the time-series index of every row (census receipt, \texttt{seal.\allowbreak{}identity\_\allowbreak{}projection\_\allowbreak{}read\_\allowbreak{}by\_\allowbreak{}unchanged\_\allowbreak{}governed\_\allowbreak{}code}) \\
AGG-PLAN & \texttt{ROUTE\_\allowbreak{}B\_\allowbreak{}PREDICTION\_\allowbreak{}PLAN\_\allowbreak{}20260927\_\allowbreak{}V1.\allowbreak{}md:\allowbreak{}106}, \texttt{:\allowbreak{}463} & none & 2026-09-27 & committed TEST aggregate: 11,279 stays at risk at L = 24 and about 750 to 1,000 events per primary under legacy definitions \\
PREPROC & \texttt{MIMIC\_\allowbreak{}IV\_\allowbreak{}READ\_\allowbreak{}SCOPING\_\allowbreak{}20260930\_\allowbreak{}V1.\allowbreak{}md:\allowbreak{}86} & none & 2026-05 & the legacy root's clip and fill quantiles, and BlendedICU's height and weight quantiles, were computed over all splits, TEST covariates included (label-free) \\
