# Supplementary material for: ICare-DT: a digital twin for continuous forecasting of intensive care patients
Source: arXiv:2611.09712 source file (2026-11-06)
Supplement: Supplementary file 19 [file s2x_disclosure_after.tex]

\textbf{Overlap with this read} (\texttt{TEST\_\allowbreak{}READ\_\allowbreak{}REGISTRY.\allowbreak{}md:\allowbreak{}142-\allowbreak{}158}):

\begin{itemize}
\item Family A. The z = 0 crossings of heart rate, respiratory rate and \spo{} have never been scored on MIMIC-IV TEST. Overlapping surfaces were scored: raw future heart and respiratory rate (TRB-M4-06), the HR $>$ 130 and \spo{} $<$ 90 threshold events (the events family of TRB-M4-02 onward), and legacy hypoxemia. Frozen eICU twins of earlier versions (A0\_dyn, A0\_dyn\_thr) were transferred zero-shot to this split in TRB-M4-07, -13, -16 and -22 (with stratified reads in -14 and -15); -16 closed negative and -22 was null after Holm, and the analysts knew these results when this zero-shot design was chosen (\texttt{MIMIC\_\allowbreak{}IV\_\allowbreak{}READ\_\allowbreak{}SCOPING\_\allowbreak{}20260930\_\allowbreak{}V1.\allowbreak{}md:\allowbreak{}83}, \texttt{icare\_\allowbreak{}dt/\allowbreak{}RESULTS.\allowbreak{}md}). C01 fine-tuned the same joint lineage on MIMIC-IV and read TEST mortality.
\item Family B. E2 (MAP below 65 mmHg in two consecutive measured hours) is word for word the legacy hypotension rule scored from TRB-M4-01 on, apart from the at-risk rule, the clock and the readout (\texttt{TEST\_\allowbreak{}READ\_\allowbreak{}REGISTRY.\allowbreak{}md:\allowbreak{}154}). Legacy KDIGO AKI (creatinine and urine output, first-6-hour baseline), legacy hypoxemia (one hour, \spo{} or SaO\textsubscript{2} below 90 or P/F below 300) and the \spo{} $<$ 90 event were scored; E3 and E4 as P0 defines them were not.
\item Secondaries (3.11). Hospital mortality (the harmonized \texttt{mortality} label, MIMIC-IV's \texttt{hospital\_\allowbreak{}expire\_\allowbreak{}flag} copied to every ICU stay of the admission) was scored on this split at landmarks 6/12/24/48 h in the legacy reads (TRB-M4-01 to -05, -07 to -19, -22 to -24; REG-5227 re-exported a job-2754 aggregate of mortality and LOS cells), among stays with LOS $\geq$ C at C = 6/12/24/48 h on the corrected clock (TRB-M4-20, scoring jobs 7436-7443, merge 7444, audit 7445) and at 24 h by C01 (REG-C01, jobs 5896-5898). Length of stay was scored at landmarks in the legacy reads and as remaining ICU LOS, LOS $-$ C among stays with LOS $\geq$ C (TRB-M4-21, jobs 7451/7452) (\texttt{TEST\_\allowbreak{}READ\_\allowbreak{}REGISTRY.\allowbreak{}md:\allowbreak{}144-\allowbreak{}145}, \texttt{:\allowbreak{}85-\allowbreak{}86}). From June 2026 every ICare-DT mortality row scored a model death CIF (ICU death with ICU discharge competing) against this hospital-death label (\texttt{TEST\_\allowbreak{}READ\_\allowbreak{}REGISTRY.\allowbreak{}md:\allowbreak{}144}, \texttt{:\allowbreak{}153}), including the zero-shot transfers of earlier frozen eICU twins (TRB-M4-07, -13, -16, -22). No listed read applied the five checkpoints of this read to MIMIC-IV TEST without refitting; REG-C01 read 24-hour mortality of MIMIC-IV fine-tunes of seed 29's lineage. No binary unit-exit-within-H label was scored before, but remaining ICU LOS at C = 48 h was (TRB-M4-21).
\item Known TEST facts: 14,211 stays; 9,804 persons over the 14,209 finite-LOS stays; 2 stays with non-finite LOS (they will carry an unresolved terminal here and be excluded from every label); legacy at-risk and event counts (AGG-PLAN); at C = 48 h, 7,016 stays of 5,446 persons with LOS $\geq$ 48 h and 1,006 hospital deaths (rate 0.143), and AUROCs of 0.876 to 0.885 for hospital death from the nine tabular models of TRB-M4-20, trained on MIMIC-IV TRAIN (corrected clock; committed scoreboard \texttt{source\_\allowbreak{}tables/\allowbreak{}revision\_\allowbreak{}v3/\allowbreak{}g3/\allowbreak{}g3\_\allowbreak{}mortality\_\allowbreak{}heldout\_\allowbreak{}scoreboard\_\allowbreak{}v1.\allowbreak{}csv}, rows \texttt{mimic4}, context 48; \texttt{G3\_\allowbreak{}LOS\_\allowbreak{}HELDOUT\_\allowbreak{}FRONTIER\_\allowbreak{}V1.\allowbreak{}md:\allowbreak{}53} gives the same 7,016 / 5,446 risk set).
\end{itemize}

Beyond ID-12997 and ID-13062, every governed dataset construction in the project reads the patient, split and source columns of every label row through the unchanged normalization verifier; these identity reads carry no covariate or outcome and are not listed one by one.

The analysts have seen the results of every read above, every eICU result the paper reports and the MIMIC-IV TRAIN census (decision 8, \texttt{ROUTE\_\allowbreak{}B\_\allowbreak{}DECISION\_\allowbreak{}20260926\_\allowbreak{}V1.\allowbreak{}md:\allowbreak{}103-\allowbreak{}106}). Route B was shaped by TEST reads (\texttt{TEST\_\allowbreak{}READ\_\allowbreak{}REGISTRY.\allowbreak{}md:\allowbreak{}138}). \texttt{sacct} on 2026-09-30 shows no job after the census 13062, so no MIMIC-IV TEST read happened after the disclosure back-fill of 2026-09-27.
