# Supplementary material for: ICare-DT: a digital twin for continuous forecasting of intensive care patients
Source: arXiv:2611.09712 source file (2026-11-06)
Supplement: Supplementary file 20 [file s2x_disclosure_intro.tex]

The canonical list below is bound by the TEST authorization (section 7.2) as the exact sorted set of its IDs. ``Scientific reads'' are the IDs beginning \texttt{REG-\allowbreak{}} or \texttt{TRB-\allowbreak{}M4-\allowbreak{}} (27); the other 7 record reconciled non-reads, identity reads, a committed aggregate and mixed-split preprocessing. A record written \texttt{:\allowbreak{}66} is line 66 of \texttt{reports/\allowbreak{}revision\_\allowbreak{}v3/\allowbreak{}TEST\_\allowbreak{}READ\_\allowbreak{}REGISTRY.\allowbreak{}md}, whose row gives the full access, selection and verification detail.
