# Supplementary material for: ICare-DT: a digital twin for continuous forecasting of intensive care patients
Source: arXiv:2611.09712 source file (2026-11-06)
Supplement: Supplementary file 21 [file s2x_jobs.tex]

M & TEST manifest (identity columns only; run from package commit A) & 13123 & 1 & 00:00:33 & COMPLETED, exit 0:0 \\
BX & Family B extract (MIMIC-IV training split only) & 13163 & 1 & 00:06:26 & COMPLETED, exit 0:0 \\
BT & Family B encoder training, arms f and g & 13164 & 10 & 00:03:19 to 00:03:36 & COMPLETED, exit 0:0 \\
BF & Family B tree fits, arms b and h & 13165 & 15 & 00:03:57 to 00:06:19 & COMPLETED, exit 0:0 \\
R & Release of the TEST observation occurrence & 13166 & 1 & 00:04:41 & COMPLETED, exit 0:0 \\
AP & Family A predictions (hours 1 to 30) & 13167 & 5 & 00:02:10 to 00:02:36 & COMPLETED, exit 0:0 \\
AS & Secondary-outcome predictions (hours 1 to 48) & 13168 & 5 & 00:01:52 to 00:02:15 & COMPLETED, exit 0:0 \\
BP & Family B predictions & 13169 & 1 & 00:02:52 & COMPLETED, exit 0:0 \\
FZ & Freeze of every prediction file & 13170 & 1 & 00:00:32 & COMPLETED, exit 0:0 \\
LB & Labels, built after the freeze & 13171 & 1 & 00:04:43 & COMPLETED, exit 0:0 \\
SC & Scoring under the read-once marker & 13172 & 1 & 00:11:14 & COMPLETED, exit 0:0 \\
VF & Verification of the scored outputs & 13173 & 1 & 00:12:05 & COMPLETED, exit 0:0 \\
