# Supplementary material for: ICare-DT: a digital twin for continuous forecasting of intensive care patients
Source: arXiv:2611.09712 source file (2026-11-06)
Supplement: Supplementary file 22 [file s2x_limitations.tex]

\begin{itemize}
\item MIMIC-IV TEST was read before (section 2.3): zero-shot transfers of earlier frozen eICU twins (TRB-M4-07, -13 to -16, -22), fine-tunes of the same joint lineage (REG-C01), the hypotension rule that E2 repeats, legacy KDIGO AKI (the analogue of E3), legacy hypoxemia (overlapping E4 and the \spo{} target), the HR $>$ 130 and \spo{} $<$ 90 events, and raw future heart and respiratory rate; the analysts know those results.
\item Family A tests transfer of the frozen eICU model under one input mapping; it does not test synchronization in a model adapted to MIMIC-IV.
\item The frozen model meets a large input shift (D16) that it was never trained on; nothing is adapted.
\item The targets are threshold crossings of the MIMIC-IV TRAIN mean in stays selected by measurement (the observation-gap censor), not clinical events; the hour-30 entry conditions the shorter settings on a longer record, and on the legacy clock a record can reach hour 30 through rows after the terminal.
\item The label and model clocks are the legacy one-based clock, not discharge-bounded; the terminal is the ceiling of the ICU LOS hours and the cause is the hospital flag (merged, so the family-A and family-B labels are unaffected; the mortality secondaries read the flag as hospital death, 3.11).
\item The legacy root's clip and fill quantiles use all splits (PREPROC).
\item The prefix view is procedural within one process: the governed loader holds the previously read TEST mortality and LOS columns in memory during prediction, and the predict processes hold label-determining hours (13 to 30 in AP, 13 to 48 in BP, and 13 to 48 in AS, which makes no family-A or family-B prediction), unused by construction and verified by the per-landmark invariance test (7.3), not physically absent. Test (iii) of 7.3 checks the predict modules' own text, not the modules they import, which include label modules.
\item The secondaries (3.11) are descriptive, with no criterion, on outcomes read on this split many times before (section 2.3), with results the analysts know. The death summary targets death in the unit before the head's crossing. MIMIC-IV records the time of in-hospital death (\texttt{admissions.\allowbreak{}deathtime}, \texttt{ROUTE\_\allowbreak{}B\_\allowbreak{}PREDICTION\_\allowbreak{}PLAN\_\allowbreak{}20260927\_\allowbreak{}V1.\allowbreak{}md:\allowbreak{}58}), but the legacy harmonized root used here keeps only \texttt{hospital\_\allowbreak{}expire\_\allowbreak{}flag}, without a time, and this read adds no exporter for it (decision item 19), so endpoint E1 stays excluded (4.1) and the death summary is scored against hospital death: MORT-W adds later in-hospital deaths of stays that left the unit alive in the window, and MORT-H has a longer window than the forecast, so neither calibration nor discrimination is on the eICU estimand (death in the unit within 48 hours, every such death counted). The exit summary targets leaving the unit before the head's crossing, not every unit exit, so it is not an estimand match for LOS-X\_H either. A mean forecast below the observed rate of MORT-W, MORT-H or LOS-X\_H therefore arises in part by construction, as the reworded eICU sentence states for eICU (9.3). The heads were trained only at origins where their target had not yet crossed; at hour 48 they are read outside those origins in every stay whose target has already been measured past the threshold, as the eICU death summary was. The death and exit summaries are the largest of target-specific CIFs, one of whose heads reads a channel that is nearly empty in MIMIC-IV (the three-head sensitivity shows its weight). The earlier MIMIC-IV results for these outcomes come from different models, clocks and, for LOS, estimands (D29, D30), and are context, not a comparator. In a final attempt the secondaries can stop while family A is scored (C12); they are then reported as stopped, not scored later.
\item Family B's comparator is an untuned fixed recipe; the P1 recipe keeps its documented learning-rate confound between f and g and its epoch cap; h uses in-sample TRAIN states.
\item E2 overlaps a rule already scored on this split; E4 is ascertained on hourly \spo{} in MIMIC-IV and on nurse charting in eICU; E4 is underpowered.
\item Family B's intervals condition on the fitted models; the primary test conditions on one tree seed (C6), and the tree-seed spread and the paired tree-seed sensitivity are reported but enter no test.
\item The power analysis rests on normal approximations, on eICU standard errors rescaled by event counts, on an approximate design effect for repeat stays, and on assumed correlations between settings and endpoints; it was not checked by resampling any real panel.
\item Family A's pass criterion is a count rule: a failed outcome can coexist with an eICU-sized gain in most settings (5.3), and a shown outcome with gains well below the eICU size.
\item The isolation arms and all causal analyses are not repeated on MIMIC-IV.
\end{itemize}
