# Supplementary material for: ICare-DT: a digital twin for continuous forecasting of intensive care patients
Source: arXiv:2611.09712 source file (2026-11-06)
Supplement: Supplementary file 23 [file s2x_pow_a.tex]

Retained & SE $\times$ 1, $\rho$ = 0 & SE $\times$ 1, $\rho$ = 0.5 & SE $\times$ 1.5, $\rho$ = 0 & SE $\times$ 1.5, $\rho$ = 0.5 \\
\midrule
\multicolumn{5}{l}{\textit{Synchronized versus hour-6 forecast (primary family)}} \\
1 & 0.97 / 0.03 / 0.00 / 0.00 & 0.97 / 0.03 / 0.00 / 0.00 & 0.69 / 0.31 / 0.00 / 0.00 & 0.72 / 0.28 / 0.00 / 0.00 \\
0.75 & 0.82 / 0.18 / 0.00 / 0.00 & 0.83 / 0.17 / 0.00 / 0.00 & 0.27 / 0.72 / 0.01 / 0.00 & 0.41 / 0.52 / 0.07 / 0.00 \\
0.5 & 0.28 / 0.72 / 0.01 / 0.00 & 0.41 / 0.52 / 0.07 / 0.00 & 0.01 / 0.40 / 0.59 / 0.00 & 0.11 / 0.34 / 0.55 / 0.00 \\
0.25 & 0.00 / 0.04 / 0.96 / 0.00 & 0.04 / 0.14 / 0.83 / 0.00 & 0.00 / 0.00 / 1.00 / 0.00 & 0.01 / 0.03 / 0.96 / 0.00 \\
0 & 0.00 / 0.00 / 0.975 / 0.025 & 0.00 / 0.00 / 0.980 / 0.020 & 0.00 / 0.00 / 0.975 / 0.025 & 0.00 / 0.00 / 0.980 / 0.020 \\
\midrule
\multicolumn{5}{l}{\textit{Synchronized forecast versus last measured value (registered secondary)}} \\
1 & 0.13 / 0.86 / 0.01 / 0.00 & 0.25 / 0.68 / 0.07 / 0.00 & 0.00 / 0.45 / 0.54 / 0.00 & 0.07 / 0.40 / 0.53 / 0.00 \\
0.75 & 0.01 / 0.69 / 0.30 / 0.00 & 0.10 / 0.51 / 0.38 / 0.00 & 0.00 / 0.06 / 0.94 / 0.00 & 0.03 / 0.16 / 0.81 / 0.00 \\
0.5 & 0.00 / 0.06 / 0.94 / 0.00 & 0.03 / 0.16 / 0.81 / 0.00 & 0.00 / 0.00 / 1.00 / 0.00 & 0.01 / 0.04 / 0.95 / 0.00 \\
0 & 0.00 / 0.00 / 0.98 / 0.02 & 0.00 / 0.00 / 0.98 / 0.02 & 0.00 / 0.00 / 0.98 / 0.02 & 0.00 / 0.00 / 0.98 / 0.02 \\
\midrule
\multicolumn{5}{l}{\textit{Heterogeneous case of the primary family: heart and respiratory rate at their full eICU-CRD gains, the three \spo{} settings at a common true gain}} \\
\spo{} true gain & SE $\times$ 1, $\rho$ = 0 & SE $\times$ 1, $\rho$ = 0.5 & SE $\times$ 1.5, $\rho$ = 0 & SE $\times$ 1.5, $\rho$ = 0.5 \\
\midrule
+0.02 & 0.01 / 0.98 / 0.00 / 0.00; 0.00 & 0.06 / 0.93 / 0.00 / 0.00; 0.00 & 0.00 / 0.95 / 0.05 / 0.00; 0.01 & 0.02 / 0.89 / 0.08 / 0.00; 0.00 \\
0 & 0.00 / 0.93 / 0.05 / 0.02; 0.07 & 0.00 / 0.94 / 0.04 / 0.02; 0.04 & 0.00 / 0.88 / 0.10 / 0.02; 0.04 & 0.00 / 0.88 / 0.10 / 0.02; 0.01 \\
$-$0.02 & 0.00 / 0.27 / 0.22 / 0.51; 0.68 & 0.00 / 0.37 / 0.19 / 0.44; 0.58 & 0.00 / 0.52 / 0.25 / 0.23; 0.23 & 0.00 / 0.62 / 0.20 / 0.18; 0.11 \\
