# Supplementary material for: ICare-DT: a digital twin for continuous forecasting of intensive care patients
Source: arXiv:2611.09712 source file (2026-11-06)
Supplement: Supplementary file 24 [file s2x_pow_a_in.tex]

Setting & eICU S2 $-$ S1 (SE) & Projected MIMIC-IV SE & eICU S2 $-$ LOCF (SE) & Projected MIMIC-IV SE \\
\midrule
\spo{} (12, 6) & +0.078 (0.0095) & 0.0097 & +0.062 (0.0093) & 0.0094 \\
\spo{} (18, 12) & +0.101 (0.0129) & 0.0132 & +0.060 (0.0131) & 0.0133 \\
\spo{} (30, 24) & +0.153 (0.0243) & 0.0262 & +0.085 (0.0208) & 0.0224 \\
Heart rate (12, 6) & +0.116 (0.0081) & 0.0110 & +0.010 (0.0034) & 0.0046 \\
Heart rate (18, 12) & +0.107 (0.0083) & 0.0123 & +0.027 (0.0047) & 0.0069 \\
Heart rate (30, 24) & +0.121 (0.0118) & 0.0183 & +0.042 (0.0089) & 0.0139 \\
Respiratory rate (12, 6) & +0.102 (0.0078) & 0.0109 & +0.048 (0.0061) & 0.0085 \\
Respiratory rate (18, 12) & +0.083 (0.0078) & 0.0137 & +0.046 (0.0075) & 0.0133 \\
Respiratory rate (30, 24) & +0.108 (0.0110) & 0.0277 & +0.049 (0.0127) & 0.0319 \\
