# Supplementary material for: ICare-DT: a digital twin for continuous forecasting of intensive care patients
Source: arXiv:2611.09712 source file (2026-11-06)
Supplement: Supplementary file 25 [file s2x_pow_b.tex]

Retained (true E2, E3 gains) & SE $\times$ 1 & SE $\times$ 1.25 & SE $\times$ 1.5 \\
\midrule
1 (+0.0042, +0.0075) & 0.93 / 0.99 / 0.93 / 0.01 & 0.80 / 0.93 / 0.77 / 0.04 & 0.64 / 0.82 / 0.60 / 0.13 \\
0.75 (+0.0031, +0.0056) & 0.75 / 0.90 / 0.71 / 0.07 & 0.56 / 0.73 / 0.49 / 0.20 & 0.42 / 0.58 / 0.34 / 0.34 \\
0.5 (+0.0021, +0.0037) & 0.42 / 0.58 / 0.34 / 0.34 & 0.29 / 0.41 / 0.21 / 0.51 & 0.22 / 0.31 / 0.14 / 0.62 \\
0.25 (+0.0010, +0.0019) & 0.14 / 0.19 / 0.07 / 0.74 & 0.10 / 0.14 / 0.05 / 0.81 & 0.09 / 0.11 / 0.04 / 0.84 \\
0 & 0.03 / 0.03 / 0.01 / 0.95 & 0.03 / 0.03 / 0.01 / 0.95 & 0.03 / 0.03 / 0.01 / 0.95 \\
