# Supplementary material for: ICare-DT: a digital twin for continuous forecasting of intensive care patients
Source: arXiv:2611.09712 source file (2026-11-06)
Supplement: Supplementary file 26 [file s2x_pow_b_in.tex]

Hypotension (E2) & 3,136 & 3,213 & +0.0042 (0.00132) & 0.00134 & $-$0.0044 (0.00176) & 0.00179 \\
Acute kidney injury (E3) & 1,762 & 2,392 & +0.0075 (0.00206) & 0.00181 & $-$0.0209 (0.00417) & 0.00365 \\
Hypoxemia (E4, secondary) & 587 & 674 & +0.0013 (0.00233) & 0.00218 & $-$0.0125 (0.00379) & 0.00355 \\
