# Supplementary material for: ICare-DT: a digital twin for continuous forecasting of intensive care patients
Source: arXiv:2611.09712 source file (2026-11-06)
Supplement: Supplementary file 27 [file s2x_prec.tex]

Setting & Assumed events & 95\% half-width of the AUROC & 95\% half-width of the observed rate \\
\midrule
MORT-H & 1,006 & 0.019 at AUROC 0.80; 0.022 at 0.70; 0.016 at 0.88 & 0.009 \\
MORT-W & 100 / 200 / 400 / 700 (unknown) & 0.060 / 0.042 / 0.030 / 0.023 at AUROC 0.80 & 0.003 / 0.004 / 0.006 / 0.008 \\
LOS-X\_H & event fraction 0.1 / 0.3 / 0.5 / 0.7 & 0.024 / 0.015 / 0.013 / 0.013 at AUROC 0.75 & 0.008 / 0.012 / 0.013 / 0.012 \\
