# Supplementary material for: ICare-DT: a digital twin for continuous forecasting of intensive care patients
Source: arXiv:2611.09712 source file (2026-11-06)
Supplement: Supplementary file 28 [file s2x_sec_main.tex]

Hospital death, unit exit within 48 h (MORT-W) & 324 & 0.047 & 0.687 & [0.657, 0.718] & [0.666, 0.708] & 0.0039 [0.0031, 0.0048] & $-$0.043 [$-$0.048, $-$0.038] & 0.155 [0.130, 0.179] \\
Hospital death (MORT-H) & 972 & 0.140 & 0.726 & [0.708, 0.744] & [0.695, 0.757] & 0.0039 [0.0031, 0.0048] & $-$0.136 [$-$0.145, $-$0.127] & 0.377 [0.354, 0.400] \\
Leaving the unit within 6 h (LOS-X6) & 784 & 0.113 & 0.808 & [0.793, 0.822] & [0.800, 0.816] & 0.091 [0.077, 0.105] & $-$0.022 [$-$0.029, $-$0.015] & 0.372 [0.348, 0.395] \\
Leaving the unit within 12 h (LOS-X12) & 1,318 & 0.190 & 0.791 & [0.779, 0.803] & [0.783, 0.799] & 0.130 [0.114, 0.146] & $-$0.059 [$-$0.068, $-$0.051] & 0.460 [0.439, 0.480] \\
Leaving the unit within 24 h (LOS-X24) & 2,237 & 0.322 & 0.767 & [0.756, 0.778] & [0.765, 0.768] & 0.195 [0.174, 0.215] & $-$0.127 [$-$0.137, $-$0.117] & 0.573 [0.566, 0.580] \\
Leaving the unit within 48 h (LOS-X48) & 3,548 & 0.510 & 0.765 & [0.754, 0.776] & [0.764, 0.766] & 0.267 [0.242, 0.291] & $-$0.244 [$-$0.255, $-$0.233] & 0.740 [0.735, 0.745] \\
