# Supplementary material for: ICare-DT: a digital twin for continuous forecasting of intensive care patients
Source: arXiv:2611.09712 source file (2026-11-06)
Supplement: Supplementary file 29 [file s2x_sec_pop.tex]

Included: record reaches hour 48 and unit stay lasts beyond it & 6,951 \\
\quad of which persons & 5,396 \\
Excluded: terminal clock at or before hour 48 & 7,193 \\
Excluded: record shorter than 48 h, terminal clock after hour 48 & 65 \\
Excluded: unresolved terminal & 2 \\
Manifest stays (sum) & 14,211 \\
\midrule
Events: hospital death, unit exit within 48 h (MORT-W) & 324 \\
Events: hospital death (MORT-H) & 972 \\
Events: leaving the unit within 6 h (LOS-X6) & 784 \\
Events: leaving the unit within 12 h (LOS-X12) & 1,318 \\
Events: leaving the unit within 24 h (LOS-X24) & 2,237 \\
Events: leaving the unit within 48 h (LOS-X48) & 3,548 \\
\midrule
Share of MORT-H events that are MORT-W events & 0.333 \\
