# Supplementary material for: ICare-DT: a digital twin for continuous forecasting of intensive care patients
Source: arXiv:2611.09712 source file (2026-11-06)
Supplement: Supplementary file 30 [file s2x_sec_rel.tex]

Hospital death, unit exit within 48 h (MORT-W) & 0.0 to 0.1 & 6,949; 0.004; 0.046 & 6,951; 0.003; 0.047 & 6,948; 0.004; 0.046 & 6,944; 0.004; 0.046 & 6,941; 0.004; 0.046 \\
 & 0.1 to 0.2 & 2; 0.110; 0.500 & -- & 3; 0.123; 0.333 & 7; 0.136; 0.857 & 10; 0.117; 0.500 \\
\midrule
Hospital death (MORT-H) & 0.0 to 0.1 & 6,949; 0.004; 0.140 & 6,951; 0.003; 0.140 & 6,948; 0.004; 0.140 & 6,944; 0.004; 0.139 & 6,941; 0.004; 0.139 \\
 & 0.1 to 0.2 & 2; 0.110; 0.500 & -- & 3; 0.123; 0.333 & 7; 0.136; 0.857 & 10; 0.117; 0.800 \\
\midrule
Leaving the unit within 6 h (LOS-X6) & 0.0 to 0.1 & 4,722; 0.030; 0.048 & 4,783; 0.029; 0.049 & 4,178; 0.029; 0.039 & 4,414; 0.031; 0.040 & 4,902; 0.029; 0.051 \\
 & 0.1 to 0.2 & 1,422; 0.144; 0.176 & 1,327; 0.143; 0.182 & 1,536; 0.146; 0.135 & 1,492; 0.144; 0.145 & 1,340; 0.143; 0.178 \\
 & 0.2 to 0.3 & 459; 0.240; 0.283 & 506; 0.241; 0.310 & 715; 0.243; 0.263 & 621; 0.239; 0.275 & 468; 0.241; 0.344 \\
 & 0.3 to 0.4 & 150; 0.351; 0.413 & 190; 0.343; 0.405 & 301; 0.344; 0.362 & 219; 0.342; 0.466 & 164; 0.342; 0.494 \\
 & 0.4 to 0.5 & 97; 0.443; 0.495 & 79; 0.444; 0.430 & 119; 0.447; 0.479 & 98; 0.445; 0.490 & 60; 0.441; 0.683 \\
 & 0.5 to 0.6 & 51; 0.546; 0.608 & 36; 0.543; 0.639 & 63; 0.540; 0.571 & 58; 0.547; 0.586 & 14; 0.544; 0.857 \\
 & 0.6 to 0.7 & 33; 0.655; 0.727 & 19; 0.631; 0.684 & 32; 0.638; 0.594 & 29; 0.640; 0.690 & 3; 0.624; 0.333 \\
 & 0.7 to 0.8 & 13; 0.734; 0.692 & 9; 0.743; 0.667 & 7; 0.734; 0.714 & 13; 0.747; 0.692 & -- \\
 & 0.8 to 0.9 & 3; 0.835; 1.000 & 2; 0.871; 0.500 & -- & 7; 0.842; 0.857 & -- \\
 & 0.9 to 1.0 & 1; 0.901; 0.000 & -- & -- & -- & -- \\
\midrule
Leaving the unit within 12 h (LOS-X12) & 0.0 to 0.1 & 3,585; 0.031; 0.066 & 3,779; 0.029; 0.071 & 3,344; 0.030; 0.059 & 3,304; 0.030; 0.054 & 3,904; 0.031; 0.074 \\
 & 0.1 to 0.2 & 1,673; 0.148; 0.203 & 1,480; 0.148; 0.224 & 1,427; 0.149; 0.195 & 1,602; 0.148; 0.185 & 1,575; 0.148; 0.244 \\
 & 0.2 to 0.3 & 1,022; 0.245; 0.374 & 963; 0.245; 0.363 & 1,208; 0.247; 0.305 & 1,122; 0.246; 0.316 & 897; 0.243; 0.363 \\
 & 0.3 to 0.4 & 387; 0.340; 0.470 & 468; 0.342; 0.466 & 610; 0.343; 0.446 & 574; 0.344; 0.469 & 413; 0.339; 0.487 \\
 & 0.4 to 0.5 & 149; 0.446; 0.597 & 160; 0.442; 0.544 & 224; 0.439; 0.513 & 199; 0.440; 0.598 & 124; 0.440; 0.694 \\
 & 0.5 to 0.6 & 71; 0.546; 0.535 & 61; 0.538; 0.541 & 91; 0.546; 0.626 & 83; 0.542; 0.627 & 33; 0.541; 0.848 \\
 & 0.6 to 0.7 & 40; 0.657; 0.775 & 27; 0.639; 0.741 & 37; 0.646; 0.649 & 43; 0.644; 0.721 & 5; 0.647; 0.600 \\
 & 0.7 to 0.8 & 19; 0.741; 0.842 & 9; 0.743; 0.778 & 10; 0.743; 0.800 & 15; 0.746; 0.867 & -- \\
 & 0.8 to 0.9 & 4; 0.838; 1.000 & 3; 0.828; 1.000 & -- & 9; 0.845; 0.778 & -- \\
 & 0.9 to 1.0 & 1; 0.909; 0.000 & 1; 0.901; 1.000 & -- & -- & -- \\
\midrule
Leaving the unit within 24 h (LOS-X24) & 0.0 to 0.1 & 2,735; 0.034; 0.105 & 2,980; 0.032; 0.115 & 2,620; 0.034; 0.095 & 2,609; 0.034; 0.095 & 3,097; 0.035; 0.121 \\
 & 0.1 to 0.2 & 1,058; 0.149; 0.303 & 1,045; 0.149; 0.353 & 991; 0.150; 0.301 & 968; 0.149; 0.299 & 1,138; 0.149; 0.363 \\
 & 0.2 to 0.3 & 1,136; 0.253; 0.437 & 1,001; 0.250; 0.429 & 1,036; 0.250; 0.412 & 1,016; 0.253; 0.415 & 1,072; 0.251; 0.450 \\
 & 0.3 to 0.4 & 1,180; 0.350; 0.508 & 1,038; 0.347; 0.512 & 1,071; 0.350; 0.489 & 1,286; 0.349; 0.474 & 1,002; 0.349; 0.538 \\
 & 0.4 to 0.5 & 610; 0.437; 0.602 & 601; 0.441; 0.612 & 831; 0.445; 0.563 & 765; 0.442; 0.579 & 498; 0.439; 0.631 \\
 & 0.5 to 0.6 & 143; 0.540; 0.650 & 204; 0.537; 0.637 & 306; 0.537; 0.667 & 202; 0.537; 0.698 & 117; 0.542; 0.752 \\
 & 0.6 to 0.7 & 52; 0.645; 0.827 & 57; 0.643; 0.772 & 75; 0.637; 0.667 & 69; 0.640; 0.783 & 23; 0.633; 0.913 \\
 & 0.7 to 0.8 & 30; 0.741; 0.800 & 19; 0.742; 0.842 & 20; 0.742; 0.850 & 23; 0.739; 0.826 & 4; 0.721; 1.000 \\
 & 0.8 to 0.9 & 6; 0.839; 1.000 & 4; 0.826; 1.000 & 1; 0.843; 1.000 & 13; 0.848; 0.769 & -- \\
 & 0.9 to 1.0 & 1; 0.916; 0.000 & 2; 0.920; 1.000 & -- & -- & -- \\
\midrule
Leaving the unit within 48 h (LOS-X48) & 0.0 to 0.1 & 2,220; 0.044; 0.207 & 2,412; 0.041; 0.226 & 2,084; 0.045; 0.197 & 2,074; 0.046; 0.184 & 2,550; 0.045; 0.233 \\
 & 0.1 to 0.2 & 882; 0.148; 0.452 & 904; 0.148; 0.482 & 883; 0.149; 0.443 & 874; 0.148; 0.475 & 1,012; 0.148; 0.529 \\
 & 0.2 to 0.3 & 860; 0.249; 0.594 & 816; 0.248; 0.604 & 853; 0.250; 0.567 & 788; 0.249; 0.553 & 866; 0.250; 0.603 \\
 & 0.3 to 0.4 & 875; 0.351; 0.673 & 814; 0.351; 0.671 & 831; 0.349; 0.649 & 858; 0.351; 0.647 & 788; 0.349; 0.708 \\
 & 0.4 to 0.5 & 861; 0.449; 0.711 & 805; 0.449; 0.727 & 849; 0.449; 0.704 & 970; 0.450; 0.693 & 814; 0.449; 0.741 \\
 & 0.5 to 0.6 & 800; 0.548; 0.759 & 724; 0.547; 0.772 & 782; 0.550; 0.752 & 888; 0.544; 0.756 & 648; 0.545; 0.762 \\
 & 0.6 to 0.7 & 378; 0.635; 0.804 & 371; 0.640; 0.784 & 523; 0.642; 0.788 & 408; 0.638; 0.828 & 237; 0.638; 0.873 \\
 & 0.7 to 0.8 & 62; 0.733; 0.871 & 94; 0.735; 0.894 & 140; 0.729; 0.864 & 76; 0.733; 0.868 & 35; 0.738; 0.943 \\
 & 0.8 to 0.9 & 11; 0.832; 1.000 & 9; 0.831; 0.778 & 6; 0.820; 0.667 & 12; 0.840; 1.000 & 1; 0.809; 1.000 \\
 & 0.9 to 1.0 & 2; 0.923; 0.500 & 2; 0.941; 1.000 & -- & 3; 0.906; 0.667 & -- \\
