# Supplementary material for: ICare-DT: a digital twin for continuous forecasting of intensive care patients
Source: arXiv:2611.09712 source file (2026-11-06)
Supplement: Supplementary file 31 [file s2x_sec_seed.tex]

\multicolumn{8}{l}{\textit{Hospital death, unit exit within 48 h (MORT-W)}} \\
\quad Seed 13 & 0.699 & 0.172 & 0.256 & 0.046 & 0.0039 & not estimable$^{\mathrm{a}}$ & not estimable$^{\mathrm{a}}$ \\
\quad Seed 17 & 0.704 & 0.137 & 0.271 & 0.046 & 0.0027 & not estimable$^{\mathrm{a}}$ & not estimable$^{\mathrm{a}}$ \\
\quad Seed 23 & 0.666 & 0.153 & 0.256 & 0.045 & 0.0044 & not estimable$^{\mathrm{a}}$ & not estimable$^{\mathrm{a}}$ \\
\quad Seed 29 & 0.693 & 0.176 & 0.254 & 0.045 & 0.0042 & not estimable$^{\mathrm{a}}$ & not estimable$^{\mathrm{a}}$ \\
\quad Seed 31 & 0.672 & 0.135 & 0.260 & 0.045 & 0.0043 & not estimable$^{\mathrm{a}}$ & not estimable$^{\mathrm{a}}$ \\
\quad Five-seed mean & 0.687 & 0.155 & 0.259 & 0.046 & 0.0039 & not estimable$^{\mathrm{b}}$ & not estimable$^{\mathrm{b}}$ \\
\quad 95\% $t$ interval & [0.666, 0.708] & [0.130, 0.179] & [0.251, 0.268] & [0.045, 0.046] & [0.0031, 0.0048] & not estimable$^{\mathrm{b}}$ & not estimable$^{\mathrm{b}}$ \\
\midrule
\multicolumn{8}{l}{\textit{Hospital death (MORT-H)}} \\
\quad Seed 13 & 0.750 & 0.402 & 0.756 & 0.137 & 0.0039 & not estimable$^{\mathrm{a}}$ & not estimable$^{\mathrm{a}}$ \\
\quad Seed 17 & 0.744 & 0.373 & 0.806 & 0.138 & 0.0027 & not estimable$^{\mathrm{a}}$ & not estimable$^{\mathrm{a}}$ \\
\quad Seed 23 & 0.692 & 0.358 & 0.766 & 0.136 & 0.0044 & not estimable$^{\mathrm{a}}$ & not estimable$^{\mathrm{a}}$ \\
\quad Seed 29 & 0.736 & 0.388 & 0.756 & 0.137 & 0.0042 & not estimable$^{\mathrm{a}}$ & not estimable$^{\mathrm{a}}$ \\
\quad Seed 31 & 0.708 & 0.362 & 0.767 & 0.137 & 0.0043 & not estimable$^{\mathrm{a}}$ & not estimable$^{\mathrm{a}}$ \\
\quad Five-seed mean & 0.726 & 0.377 & 0.770 & 0.137 & 0.0039 & not estimable$^{\mathrm{b}}$ & not estimable$^{\mathrm{b}}$ \\
\quad 95\% $t$ interval & [0.695, 0.757] & [0.354, 0.400] & [0.745, 0.796] & [0.136, 0.138] & [0.0031, 0.0048] & not estimable$^{\mathrm{b}}$ & not estimable$^{\mathrm{b}}$ \\
\midrule
\multicolumn{8}{l}{\textit{Leaving the unit within 6 h (LOS-X6)}} \\
\quad Seed 13 & 0.807 & 0.373 & 0.289 & 0.085 & 0.089 & 0.12 & 0.89 \\
\quad Seed 17 & 0.802 & 0.347 & 0.296 & 0.087 & 0.085 & 0.07 & 0.84 \\
\quad Seed 23 & 0.806 & 0.361 & 0.287 & 0.085 & 0.106 & $-$0.06 & 0.91 \\
\quad Seed 29 & 0.819 & 0.396 & 0.280 & 0.083 & 0.098 & 0.17 & 0.99 \\
\quad Seed 31 & 0.807 & 0.381 & 0.295 & 0.087 & 0.078 & 0.37 & 0.95 \\
\quad Five-seed mean & 0.808 & 0.372 & 0.289 & 0.086 & 0.091 & 0.13 & 0.92 \\
\quad 95\% $t$ interval & [0.800, 0.816] & [0.348, 0.395] & [0.281, 0.297] & [0.084, 0.087] & [0.077, 0.105] & [$-$0.06, 0.33] & [0.84, 0.99] \\
\midrule
\multicolumn{8}{l}{\textit{Leaving the unit within 12 h (LOS-X12)}} \\
\quad Seed 13 & 0.795 & 0.466 & 0.413 & 0.132 & 0.128 & 0.43 & 0.92 \\
\quad Seed 17 & 0.786 & 0.444 & 0.424 & 0.134 & 0.123 & 0.33 & 0.83 \\
\quad Seed 23 & 0.787 & 0.443 & 0.410 & 0.131 & 0.144 & 0.23 & 0.88 \\
\quad Seed 29 & 0.801 & 0.482 & 0.401 & 0.128 & 0.142 & 0.36 & 0.96 \\
\quad Seed 31 & 0.787 & 0.464 & 0.429 & 0.136 & 0.113 & 0.53 & 0.89 \\
\quad Five-seed mean & 0.791 & 0.460 & 0.415 & 0.132 & 0.130 & 0.38 & 0.90 \\
\quad 95\% $t$ interval & [0.783, 0.799] & [0.439, 0.480] & [0.401, 0.430] & [0.128, 0.136] & [0.114, 0.146] & [0.23, 0.52] & [0.83, 0.96] \\
\midrule
\multicolumn{8}{l}{\textit{Leaving the unit within 24 h (LOS-X24)}} \\
\quad Seed 13 & 0.768 & 0.572 & 0.581 & 0.196 & 0.195 & 0.61 & 0.81 \\
\quad Seed 17 & 0.765 & 0.569 & 0.601 & 0.199 & 0.186 & 0.58 & 0.74 \\
\quad Seed 23 & 0.766 & 0.566 & 0.569 & 0.192 & 0.211 & 0.49 & 0.80 \\
\quad Seed 29 & 0.768 & 0.576 & 0.567 & 0.191 & 0.210 & 0.52 & 0.82 \\
\quad Seed 31 & 0.768 & 0.581 & 0.610 & 0.204 & 0.172 & 0.74 & 0.80 \\
\quad Five-seed mean & 0.767 & 0.573 & 0.586 & 0.196 & 0.195 & 0.59 & 0.79 \\
\quad 95\% $t$ interval & [0.765, 0.768] & [0.566, 0.580] & [0.562, 0.609] & [0.190, 0.203] & [0.174, 0.215] & [0.47, 0.71] & [0.75, 0.83] \\
\midrule
\multicolumn{8}{l}{\textit{Leaving the unit within 48 h (LOS-X48)}} \\
\quad Seed 13 & 0.766 & 0.739 & 0.757 & 0.260 & 0.269 & 1.13 & 0.78 \\
\quad Seed 17 & 0.764 & 0.739 & 0.787 & 0.266 & 0.258 & 1.15 & 0.73 \\
\quad Seed 23 & 0.764 & 0.735 & 0.734 & 0.252 & 0.285 & 1.04 & 0.77 \\
\quad Seed 29 & 0.766 & 0.742 & 0.730 & 0.251 & 0.284 & 1.07 & 0.80 \\
\quad Seed 31 & 0.765 & 0.745 & 0.815 & 0.278 & 0.238 & 1.30 & 0.78 \\
\quad Five-seed mean & 0.765 & 0.740 & 0.765 & 0.261 & 0.267 & 1.14 & 0.77 \\
\quad 95\% $t$ interval & [0.764, 0.766] & [0.735, 0.745] & [0.720, 0.810] & [0.248, 0.275] & [0.242, 0.291] & [1.01, 1.26] & [0.74, 0.80] \\
