# Supplementary material for: ICare-DT: a digital twin for continuous forecasting of intensive care patients
Source: arXiv:2611.09712 source file (2026-11-06)
Supplement: Supplementary file 32 [file s2x_sec_seedmech.tex]

Exit-forecast sums set to 1 & 0 & 0 & 0 & 0 & 0 \\
\midrule
Death forecast $P_D$, 5th percentile & 0.00033 & 0.00029 & 0.00044 & 0.00040 & 0.00047 \\
Death forecast $P_D$, 25th percentile & 0.00065 & 0.00057 & 0.00092 & 0.00079 & 0.00087 \\
Death forecast $P_D$, 50th percentile & 0.0012 & 0.0010 & 0.0015 & 0.0014 & 0.0014 \\
Death forecast $P_D$, 75th percentile & 0.0030 & 0.0022 & 0.0028 & 0.0030 & 0.0026 \\
Death forecast $P_D$, 95th percentile & 0.019 & 0.012 & 0.021 & 0.017 & 0.020 \\
\midrule
Exit forecast $P_X(48)$, 5th percentile & 0.024 & 0.020 & 0.023 & 0.025 & 0.022 \\
Exit forecast $P_X(48)$, 25th percentile & 0.062 & 0.051 & 0.072 & 0.071 & 0.054 \\
Exit forecast $P_X(48)$, 50th percentile & 0.24 & 0.22 & 0.26 & 0.27 & 0.19 \\
Exit forecast $P_X(48)$, 75th percentile & 0.44 & 0.43 & 0.47 & 0.47 & 0.40 \\
Exit forecast $P_X(48)$, 95th percentile & 0.61 & 0.62 & 0.65 & 0.62 & 0.58 \\
\midrule
$P_D$ attained by the heart-rate head (\%) & 7.8 & 17.3 & 1.6 & 21.7 & 31.0 \\
$P_D$ attained by the respiratory-rate head (\%) & 11.9 & 54.6 & 36.4 & 21.3 & 4.7 \\
$P_D$ attained by the \spo{} head (\%) & 79.4 & 27.9 & 61.9 & 56.9 & 63.2 \\
$P_D$ attained by the SaO\textsubscript{2} head (\%) & 0.9 & 0.1 & 0.0 & 0.0 & 1.1 \\
\midrule
$P_X(48)$ attained by the heart-rate head (\%) & 50.9 & 46.1 & 49.3 & 50.7 & 52.5 \\
$P_X(48)$ attained by the respiratory-rate head (\%) & 17.9 & 31.7 & 30.6 & 23.8 & 29.7 \\
$P_X(48)$ attained by the \spo{} head (\%) & 10.0 & 6.1 & 10.4 & 14.0 & 2.1 \\
$P_X(48)$ attained by the SaO\textsubscript{2} head (\%) & 21.2 & 16.1 & 9.8 & 11.5 & 15.7 \\
