# Supplementary material for: ICare-DT: a digital twin for continuous forecasting of intensive care patients
Source: arXiv:2611.09712 source file (2026-11-06)
Supplement: Supplementary file 33 [file s2x_sec_three.tex]

Hospital death, unit exit within 48 h (MORT-W) & 0.687 & 0.687 [0.666, 0.708] & 0.155 [0.130, 0.179] & 0.0039 [0.0030, 0.0048] & not estimable$^{\mathrm{b}}$ & not estimable$^{\mathrm{b}}$ \\
Hospital death (MORT-H) & 0.726 & 0.726 [0.695, 0.757] & 0.377 [0.354, 0.400] & 0.0039 [0.0030, 0.0048] & not estimable$^{\mathrm{b}}$ & not estimable$^{\mathrm{b}}$ \\
Leaving the unit within 6 h (LOS-X6) & 0.808 & 0.808 [0.800, 0.816] & 0.371 [0.347, 0.395] & 0.089 [0.075, 0.104] & 0.13 [$-$0.06, 0.32] & 0.90 [0.82, 0.98] \\
Leaving the unit within 12 h (LOS-X12) & 0.791 & 0.790 [0.782, 0.799] & 0.457 [0.436, 0.479] & 0.127 [0.110, 0.144] & 0.38 [0.24, 0.53] & 0.88 [0.81, 0.95] \\
Leaving the unit within 24 h (LOS-X24) & 0.767 & 0.766 [0.764, 0.767] & 0.571 [0.564, 0.578] & 0.191 [0.170, 0.213] & 0.60 [0.47, 0.72] & 0.78 [0.74, 0.83] \\
Leaving the unit within 48 h (LOS-X48) & 0.765 & 0.763 [0.762, 0.765] & 0.739 [0.734, 0.743] & 0.263 [0.238, 0.288] & 1.15 [1.02, 1.27] & 0.76 [0.73, 0.80] \\
