# Supplementary material for: ICare-DT: a digital twin for continuous forecasting of intensive care patients
Source: arXiv:2611.09712 source file (2026-11-06)
Supplement: Supplementary file 34 [file s2x_trb20.tex]

\multicolumn{8}{l}{7,016 test stays of 5,446 persons with an ICU length of stay of at least 48 h (corrected clock); 1,006 hospital deaths (rate 0.143)} \\
\midrule
\texttt{lgbm\_\allowbreak{}leaf31\_\allowbreak{}v1} & 0.882 & 0.603 & 0.273 & 0.083 & 0.088 & 1.038 & $-$0.0034 \\
\texttt{lgbm\_\allowbreak{}leaf15\_\allowbreak{}v1} & 0.883 & 0.603 & 0.272 & 0.083 & 0.094 & 1.065 & $-$0.0012 \\
\texttt{xgb\_\allowbreak{}depth4\_\allowbreak{}v1} & 0.884 & 0.605 & 0.271 & 0.083 & 0.051 & 1.032 & $-$0.0010 \\
\texttt{xgb\_\allowbreak{}depth6\_\allowbreak{}v1} & 0.884 & 0.609 & 0.271 & 0.083 & 0.075 & 1.020 & $-$0.0041 \\
\texttt{catboost\_\allowbreak{}depth6\_\allowbreak{}v1} & 0.881 & 0.604 & 0.274 & 0.083 & 0.164 & 1.134 & +0.0003 \\
\texttt{catboost\_\allowbreak{}depth8\_\allowbreak{}v1} & 0.881 & 0.605 & 0.274 & 0.083 & 0.172 & 1.127 & $-$0.0012 \\
\texttt{ridge\_\allowbreak{}logit\_\allowbreak{}stack\_\allowbreak{}all6\_\allowbreak{}train\_\allowbreak{}oof\_\allowbreak{}v1} & 0.885 & 0.612 & 0.270 & 0.082 & $-$0.034 & 0.995 & +0.0023 \\
\texttt{nested\_\allowbreak{}shrinkage\_\allowbreak{}train\_\allowbreak{}only\_\allowbreak{}v1} & 0.884 & 0.610 & 0.270 & 0.082 & 0.006 & 1.012 & +0.0006 \\
\texttt{tabm\_\allowbreak{}0p0p3\_\allowbreak{}registered\_\allowbreak{}v1} & 0.876 & 0.583 & 0.279 & 0.085 & $-$0.048 & 0.946 & $-$0.0012 \\
