# Supplementary material for: ICare-DT: a digital twin for continuous forecasting of intensive care patients
Source: arXiv:2611.09712 source file (2026-11-06)
Supplement: Supplementary file 35 [file s2x_trb21.tex]

\multicolumn{3}{l}{7,016 test stays of 5,446 persons with an ICU length of stay of at least 48 h (corrected clock)} \\
\multicolumn{3}{l}{Models fitted on 32,364 training stays of 24,998 persons} \\
\midrule
\texttt{frozen\_\allowbreak{}component\_\allowbreak{}log1p\_\allowbreak{}lgbm\_\allowbreak{}v1} & 67.8 & 326 \\
\texttt{frozen\_\allowbreak{}component\_\allowbreak{}raw\_\allowbreak{}lgbm\_\allowbreak{}v1} & 68.2 & 326 \\
\texttt{frozen\_\allowbreak{}component\_\allowbreak{}sqrt1p\_\allowbreak{}lgbm\_\allowbreak{}v1} & 68.1 & 326 \\
\texttt{frozen\_\allowbreak{}component\_\allowbreak{}xgboost\_\allowbreak{}lognormal\_\allowbreak{}aft\_\allowbreak{}v1} & 68.1 & 326 \\
\texttt{frozen\_\allowbreak{}oof\_\allowbreak{}simplex\_\allowbreak{}cell\_\allowbreak{}median\_\allowbreak{}calibrated\_\allowbreak{}v1} & 67.7 & 326 \\
\texttt{frozen\_\allowbreak{}oof\_\allowbreak{}simplex\_\allowbreak{}stack\_\allowbreak{}v1} & 67.7 & 326 \\
\texttt{registered\_\allowbreak{}catboost\_\allowbreak{}mae\_\allowbreak{}seed20260826\_\allowbreak{}v1} & 69.6 & 326 \\
\texttt{registered\_\allowbreak{}constant\_\allowbreak{}train\_\allowbreak{}median\_\allowbreak{}v1} & 82.4 & 0 \\
\texttt{registered\_\allowbreak{}equal\_\allowbreak{}weight\_\allowbreak{}raw\_\allowbreak{}cat\_\allowbreak{}xgb\_\allowbreak{}log\_\allowbreak{}v1} & 68.4 & 326 \\
\texttt{registered\_\allowbreak{}lgbm\_\allowbreak{}recent\_\allowbreak{}log1p\_\allowbreak{}l1\_\allowbreak{}seed20260826\_\allowbreak{}v1} & 67.9 & 326 \\
\texttt{registered\_\allowbreak{}lgbm\_\allowbreak{}recent\_\allowbreak{}raw\_\allowbreak{}l1\_\allowbreak{}seed13\_\allowbreak{}v1} & 68.2 & 326 \\
\texttt{registered\_\allowbreak{}lgbm\_\allowbreak{}static\_\allowbreak{}l1\_\allowbreak{}seed13\_\allowbreak{}v1} & 80.8 & 4 \\
\texttt{registered\_\allowbreak{}xgboost\_\allowbreak{}absoluteerror\_\allowbreak{}seed20260826\_\allowbreak{}v1} & 68.6 & 326 \\
