# Supplementary material for: ICare-DT: a digital twin for continuous forecasting of intensive care patients
Source: arXiv:2611.09712 source file (2026-11-06)
Supplement: Supplementary file 36 [file s3_registered.tex]

Synthetic tapes & History-blind & 0.520 [0.486, 0.551] & -- & yes \\
Synthetic tapes & Dosing-window means & 0.592 [0.560, 0.620] & +0.072 [+0.043, +0.101] & yes \\
Synthetic tapes & Assimilating & 0.667 [0.640, 0.690] & +0.147 [+0.113, +0.182] & yes \\
Synthetic tapes & Occupancy contrast & 0.600 [0.571, 0.629] & +0.079 [+0.039, +0.123] & yes \\
Synthetic tapes & Cadence-aware & 0.461 [0.421, 0.500] & -0.059 [-0.106, -0.009] & yes \\
Synthetic tapes & Oracle (true trait) & 0.802 [0.780, 0.823] & -- & yes \\
\midrule
Real, hourly observed & History-blind & 0.219 [0.159, 0.274] & -- & yes \\
Real, hourly observed & Dosing-window means & 0.252 [0.190, 0.311] & +0.033 [-0.015, +0.076] & yes \\
Real, hourly observed & Assimilating & 0.358 [0.308, 0.404] & +0.139 [+0.082, +0.200] & yes \\
Real, hourly observed & Occupancy contrast & 0.310 [0.261, 0.354] & +0.091 [+0.027, +0.157] & yes \\
Real, hourly observed & Cadence-aware & 0.369 [0.328, 0.406] & +0.150 [+0.082, +0.220] & yes \\
Real, hourly observed & Oracle (true trait) & 0.802 [0.780, 0.823] & -- & yes \\
\midrule
Real cadence, discovery & History-blind & 0.036 [0.005, 0.064] & -- & no \\
Real cadence, discovery & Dosing-window means & 0.066 [0.019, 0.111] & +0.030 [-0.000, +0.060] & no \\
Real cadence, discovery & Assimilating & 0.060 [0.025, 0.090] & +0.024 [-0.011, +0.057] & no \\
Real cadence, discovery & Occupancy contrast & 0.064 [0.031, 0.094] & +0.028 [-0.013, +0.068] & no \\
Real cadence, discovery & Cadence-aware & 0.181 [0.137, 0.221] & +0.144 [+0.094, +0.193] & yes \\
Real cadence, discovery & Oracle (true trait) & 0.802 [0.780, 0.823] & -- & yes \\
\midrule
Real cadence, replication & History-blind & 0.056 [0.018, 0.092] & -- & no \\
Real cadence, replication & Dosing-window means & 0.117 [0.065, 0.166] & +0.061 [+0.029, +0.091] & no \\
Real cadence, replication & Assimilating & 0.052 [0.009, 0.092] & -0.004 [-0.043, +0.034] & no \\
Real cadence, replication & Occupancy contrast & 0.051 [0.015, 0.082] & -0.005 [-0.051, +0.037] & no \\
Real cadence, replication & Cadence-aware & 0.170 [0.113, 0.220] & +0.114 [+0.054, +0.167] & yes \\
Real cadence, replication & Oracle (true trait) & 0.803 [0.780, 0.824] & -- & yes \\
\midrule
Real cadence, fixed schedule & History-blind & 0.089 [0.034, 0.141] & -- & no \\
Real cadence, fixed schedule & Dosing-window means & 0.110 [0.062, 0.158] & +0.021 [-0.016, +0.060] & no \\
Real cadence, fixed schedule & Assimilating & 0.112 [0.068, 0.153] & +0.023 [-0.019, +0.065] & no \\
Real cadence, fixed schedule & Occupancy contrast & 0.110 [0.067, 0.148] & +0.021 [-0.024, +0.066] & no \\
Real cadence, fixed schedule & Cadence-aware & 0.129 [0.062, 0.186] & +0.040 [-0.020, +0.095] & no \\
Real cadence, fixed schedule & Oracle (true trait) & 0.805 [0.782, 0.825] & -- & yes \\
