# Supplementary material for: ICare-DT: a digital twin for continuous forecasting of intensive care patients
Source: arXiv:2611.09712 source file (2026-11-06)
Supplement: Supplementary file 37 [file s4_learners.tex]

S-learner (boosting) & 0.232 & 0.08 & 0.231 & 0.10 & 0.232 & 0.03 \\
T-learner (boosting) & 0.353 & 0.01 & 0.348 & 0.12 & 0.344 & -0.00 \\
X-learner (boosting) & 0.328 & -0.05 & 0.260 & 0.11 & 0.251 & -0.03 \\
DR-learner (boosting) & 0.291 & 0.03 & 0.276 & 0.02 & 0.295 & -0.01 \\
DR-learner (ridge) & 0.523 & 0.03 & 0.592 & 0.06 & 0.385 & 0.03 \\
R-learner (boosting) & 0.530 & 0.01 & 0.380 & 0.05 & 0.878 & -0.07 \\
R-learner (ridge) & 0.345 & 0.05 & 0.358 & 0.06 & 0.308 & 0.01 \\
Causal forest & 0.248 & -0.09 & 0.241 & 0.09 & 0.593 & -0.04 \\
TARNet & 0.482 & 0.02 & 0.395 & 0.02 & 0.349 & 0.05 \\
DragonNet & 0.467 & 0.04 & 0.404 & 0.01 & 0.367 & 0.09 \\
Random-slope lag model & 0.546 & 0.26 & 0.574 & 0.25 & 0.412 & 0.20 \\
Random-slope lag model (kernel-informed) & 0.572 & 0.31 & 0.603 & 0.28 & 0.795 & 0.21 \\
Causal forest (kernel-informed) & 0.240 & -0.03 & 0.247 & 0.02 & 2.213 & 0.04 \\
Causal Transformer & 0.239 & 0.03 & 0.235 & 0.04 & 0.238 & 0.03 \\
RMSN & 0.245 & -0.01 & 0.245 & -0.01 & 0.246 & 0.04 \\
G-Net (Causal Transformer code) & 0.241 & 0.05 & 0.238 & 0.10 & 0.248 & 0.04 \\
CRN (failed its synthetic gate) & 0.242 & -0.01 & 0.240 & -0.01 & 0.242 & 0.03 \\
Linear response model (structure-informed) & 0.189 & 0.58 & 0.179 & 0.64 & 0.193 & 0.56 \\
Oracle-structure learner (factual data) & 0.189 & 0.58 & 0.179 & 0.65 & 0.194 & 0.55 \\
Population prior only & 0.232 & -0.00 & 0.232 & -0.02 & 0.232 & 0.04 \\
Predict zero & 0.232 & -- & 0.232 & -- & 0.232 & -- \\
\midrule
SD of true effect & 0.232 & -- & 0.232 & -- & 0.232 & -- \\
