# Supplementary material for: ICare-DT: a digital twin for continuous forecasting of intensive care patients
Source: arXiv:2611.09712 source file (2026-11-06)
Supplement: Supplementary file 38 [file s5_icare_rh.tex]

Registered scenario & in family & 0.227 & 0.786 & 0.141 & -0.086 [-0.100, -0.073] \\
New seed & in family & 0.212 & 0.788 & 0.131 & -0.082 [-0.093, -0.070] \\
Slower washout (decay 0.6) & in family & 0.209 & 0.789 & 0.128 & -0.081 [-0.092, -0.069] \\
Decay 0.73 & in family & 0.221 & 0.788 & 0.136 & -0.084 [-0.096, -0.072] \\
Lag 3 h & in family & 0.204 & 0.796 & 0.124 & -0.080 [-0.092, -0.069] \\
Fixed schedule & in family & 0.227 & 0.790 & 0.139 & -0.088 [-0.100, -0.075] \\
Linear route shape & in family & 0.227 & 0.793 & 0.138 & -0.089 [-0.102, -0.076] \\
Earlier query (hour 30) & in family & 0.147 & 0.640 & 0.113 & -0.034 [-0.043, -0.025] \\
AR(2) baseline with drift & out of family & 0.227 & 0.813 & 0.136 & -0.090 [-0.100, -0.079] \\
Level shifts & out of family & 0.227 & 0.766 & 0.146 & -0.081 [-0.094, -0.068] \\
Heavy-tailed noise (t, 3 df) & out of family & 0.227 & 0.770 & 0.146 & -0.081 [-0.094, -0.067] \\
Clipped trait prior & out of family & 0.199 & 0.745 & 0.133 & -0.066 [-0.077, -0.055] \\
Linear response route & out of family & 0.252 & 0.817 & 0.146 & -0.106 [-0.123, -0.090] \\
Hill response (n = 2) & out of family & 0.257 & 0.841 & 0.139 & -0.118 [-0.131, -0.103] \\
Two-compartment kinetics & out of family & 0.157 & 0.645 & 0.121 & -0.037 [-0.043, -0.030] \\
Drifting gain & out of family & 0.195 & 0.493 & 0.183 & -0.012 [-0.026, +0.002] \\
