# Supplementary material for: ICare-DT: a digital twin for continuous forecasting of intensive care patients
Source: arXiv:2611.09712 source file (2026-11-06)
Supplement: Supplementary file 39 [file s6_sync.tex]

Heart rate, 12 h, next 6 h & 6648 & +0.116$^{*}$ & +0.010$^{*}$ & +0.118$^{*}$ & +0.170$^{*}$ & -0.011$^{*}$ \\
Heart rate, 18 h, next 12 h & 4668 & +0.107$^{*}$ & +0.027$^{*}$ & +0.133$^{*}$ & +0.185$^{*}$ & -0.003 \\
Heart rate, 30 h, next 24 h & 2141 & +0.121$^{*}$ & +0.042$^{*}$ & +0.118$^{*}$ & +0.160$^{*}$ & +0.010 \\
Resp. rate, 12 h, next 6 h & 6117 & +0.102$^{*}$ & +0.048$^{*}$ & +0.106$^{*}$ & +0.131$^{*}$ & +0.005 \\
Resp. rate, 18 h, next 12 h & 3998 & +0.083$^{*}$ & +0.046$^{*}$ & +0.146$^{*}$ & +0.154$^{*}$ & +0.000 \\
Resp. rate, 30 h, next 24 h & 1763 & +0.108$^{*}$ & +0.049$^{*}$ & +0.131$^{*}$ & +0.142$^{*}$ & +0.007 \\
SpO\textsubscript{2}, 12 h, next 6 h & 2487 & +0.078$^{*}$ & +0.062$^{*}$ & +0.090$^{*}$ & +0.128$^{*}$ & -0.006 \\
SpO\textsubscript{2}, 18 h, next 12 h & 1381 & +0.101$^{*}$ & +0.060$^{*}$ & +0.080$^{*}$ & +0.111$^{*}$ & -0.004 \\
SpO\textsubscript{2}, 30 h, next 24 h & 592 & +0.153$^{*}$ & +0.085$^{*}$ & +0.142$^{*}$ & +0.131$^{*}$ & -0.001 \\
SaO\textsubscript{2}, 12 h, next 6 h & 5699 & +0.073$^{*}$ & +0.023$^{*}$ & +0.088$^{*}$ & +0.121$^{*}$ & -0.015$^{*}$ \\
SaO\textsubscript{2}, 18 h, next 12 h & 3571 & +0.083$^{*}$ & +0.025$^{*}$ & +0.100$^{*}$ & +0.136$^{*}$ & -0.017 \\
SaO\textsubscript{2}, 30 h, next 24 h & 1637 & +0.136$^{*}$ & +0.017 & +0.124$^{*}$ & +0.150$^{*}$ & +0.012 \\
