# Supplementary material for: ICare-DT: a digital twin for continuous forecasting of intensive care patients
Source: arXiv:2611.09712 source file (2026-11-06)
Supplement: Supplementary file 40 [file s7_subgroups.tex]

Age (years) & <45 & 15 & 0.758 & 0.608 to 0.860 & 0.857 [0.777, 0.922] \\
Age (years) & 45--54 & 13 & 0.736 & 0.597 to 0.875 & 0.871 [0.754, 0.956] \\
Age (years) & 55--64 & 16 & 0.717 & 0.656 to 0.890 & 0.890 [0.836, 0.934] \\
Age (years) & 65--74 & 16 & 0.700 & 0.460 to 0.821 & 0.802 [0.745, 0.857] \\
Age (years) & 75--84 & 16 & 0.702 & 0.587 to 0.844 & 0.803 [0.747, 0.857] \\
Age (years) & 85+ & 12 & 0.770 & 0.609 to 0.910 & 0.771 [0.674, 0.853] \\
\midrule
Sex & Female & 17 & 0.690 & 0.621 to 0.819 & 0.824 [0.781, 0.863] \\
Sex & Male & 17 & 0.703 & 0.621 to 0.830 & 0.813 [0.771, 0.850] \\
\midrule
Unit type & Cardiac & 13 & 0.699 & 0.583 to 0.838 & 0.814 [0.745, 0.880] \\
Unit type & Medical & 12 & 0.744 & 0.577 to 0.854 & 0.812 [0.719, 0.897] \\
Unit type & Medical-Surgical & 17 & 0.706 & 0.547 to 0.850 & 0.809 [0.774, 0.846] \\
Unit type & Neurological & 17 & 0.735 & 0.663 to 0.798 & 0.798 [0.687, 0.906] \\
Unit type & Surgical & 15 & 0.715 & 0.526 to 0.871 & 0.878 [0.807, 0.939] \\
