# Supplementary material for: ICare-DT: a digital twin for continuous forecasting of intensive care patients
Source: arXiv:2611.09712 source file (2026-11-06)
Supplement: Supplementary file 41 [file s8_net_benefit.tex]

ICU death & 48 & 0.026 & 0.03 to 0.15 & 13 of 50 \\
Heart rate & 6 & 0.066 & 0.01 to 0.48 & 48 of 50 \\
Heart rate & 12 & 0.118 & 0.01 to 0.50 & 49 of 50 \\
Heart rate & 24 & 0.245 & 0.02 to 0.50 & 49 of 50 \\
Heart rate & 48 & 0.444 & 0.04 to 0.50 & 20 of 50 \\
Respiratory rate & 6 & 0.098 & 0.01 to 0.49 & 49 of 50 \\
Respiratory rate & 12 & 0.198 & 0.02 to 0.50 & 48 of 50 \\
Respiratory rate & 24 & 0.356 & 0.04 to 0.50 & 46 of 50 \\
Respiratory rate & 48 & 0.584 & 0.07 to 0.12 & 6 of 50 \\
SpO\textsubscript{2} & 6 & 0.173 & 0.04 to 0.45 & 27 of 50 \\
SpO\textsubscript{2} & 12 & 0.342 & 0.08 to 0.49 & 39 of 50 \\
SpO\textsubscript{2} & 24 & 0.584 & 0.18 to 0.42 & 11 of 50 \\
SpO\textsubscript{2} & 48 & 0.815 & 0.44 to 0.47 & 4 of 50 \\
SaO\textsubscript{2} & 6 & 0.149 & 0.02 to 0.50 & 49 of 50 \\
SaO\textsubscript{2} & 12 & 0.262 & 0.06 to 0.50 & 45 of 50 \\
SaO\textsubscript{2} & 24 & 0.476 & 0.11 to 0.50 & 39 of 50 \\
SaO\textsubscript{2} & 48 & 0.686 & 0.21 to 0.22 & 2 of 50 \\
