# Supplementary material for: ICare-DT: a digital twin for continuous forecasting of intensive care patients
Source: arXiv:2611.09712 source file (2026-11-06)
Supplement: Supplementary file 42 [file s9_direct_route.tex]

Mean arterial pressure & 0 & +0.415 & +0.269 & +0.255 & 0 \\
\spo{} & 0 & +0.765 & 0 & +0.122 & +0.119 \\
Lactate & 0 & -0.291 & 0 & -0.175 & -0.466 \\
Heart rate & -0.230 & 0 & -0.228 & 0 & -0.121 \\
Respiratory rate & 0 & -0.261 & -0.270 & -0.145 & 0 \\
Urine output & 0 & +0.437 & +0.111 & +0.636 & +0.019 \\
Creatinine & 0 & -0.812 & 0 & 0 & -0.158 \\
pH & +0.173 & 0 & 0 & 0 & +0.286 \\
White cell count & -0.050 & 0 & -0.140 & 0 & 0 \\
Platelets & -0.184 & -0.143 & -0.304 & -0.312 & 0 \\
Bilirubin & 0 & -0.326 & -0.110 & -0.048 & 0 \\
Temperature & 0 & 0 & 0 & 0 & 0 \\
